# Supplementary material for: A statistically significant lack of debris discs in medium separation binary systems
Source: arXiv:1907.04800 ancillary file (2019-07-11)
Supplement: Supplementary file 1 [file table1.pdf]

Full version of Table 1

| Name      | Source      | Distance / pc | Component | Grade | VB6 $a''$ | VB6 $a$ / au | VB6 $e$ | Source $a$ / au | Source $e$ |
|-----------|-------------|---------------|-----------|-------|-----------|--------------|---------|-----------------|------------|
| HD 38     | Rodriguez15 | 11.3          | AB        | 4     | 11.7613   | 132.99       | 0.4973  | 68.2            |            |
| HD 123    | Drake       | 21.5          | AB        | 2     | 1.44      | 30.93        | 0.45    |                 |            |
| HD 661    | Trilling07  | 70.4          | AB        | 5     | 2.762     | 194.51       | 0.487   | 46.5            |            |
| HD 1237   | Rodriguez15 | 17.5          | AB        |       |           |              |         | 67.5            |            |
| HD 1326   | Rodriguez15 | 3.6           | AB        | 5     | 26.73     | 95.89        | 0.59    | 147.3           |            |
| HD 1404   | Rodriguez15 | 41.3          | AB        |       |           |              |         | 272             |            |
| HD 2475   | Kennedy     | 32.2          | AB        | 1     | 0.202     | 6.5          | 0.005   |                 |            |
| HD 3196   | Rodriguez15 | 21.3          | AB-C      | 1     | 0.241     | 5.12         | 0.773   | 3.95            | 0.76       |
|           |             |               | AB        |       |           |              |         | 0.035           |            |
| HD 3405   | Drake       | 44.4          | AB        |       |           |              |         | 0.053           |            |
| HD 3443   | Rodriguez15 | 15.4          | AB        | 1     | 0.675     | 10.4         | 0.218   | 8.93            | 0.24       |
| HD 3651   | Rodriguez15 | 11.1          | AB        |       |           |              |         | 474             |            |
| HD 4391   | Rodriguez15 | 15.2          | AB        |       |           |              |         | 252             |            |
|           |             |               | AC        |       |           |              |         | 743             |            |
| HD 4676   | Rodriguez15 | 23.5          | AB        | 8     | 0.006527  | 0.15         | 0.2376  | 0.126           | 0.24       |
|           |             |               | AB-C      |       |           |              |         | 5.86            |            |
| HD 4747   | Rodriguez15 | 18.7          | AB        |       |           |              |         | 7.23            | 0.64       |
| HD 4967   | Rodriguez15 | 15.6          | AB        |       |           |              |         | 262             |            |
| HD 5303   | Drake       | 88            | AB        |       |           |              |         | 0.047           |            |
| HD 6767   | Trilling07  | 56.9          | AB        | 2     | 0.2396    | 13.64        | 0.424   | 12.1            |            |
| HD 7439   | Rodriguez15 | 23.4          | AB        |       |           |              |         | 1162            |            |
| HD 7700   | Drake       | 71.7          | AB        |       |           |              |         | 0.018           |            |
| HD 7788   | Rodriguez15 | 21            | AB        | 5     | 5.96      | 124.9        | 0.384   | 106.7           |            |
|           |             |               | CD        |       |           |              |         | 18.11           | 0.04       |
|           |             |               | AB-CD     |       |           |              |         | 6734            |            |
| HD 8224   | Trilling07  | 49.3          | AB        |       |           |              |         | 128             |            |
| HD 8357   | Drake       | 44.3          | AB        |       |           |              |         | 0.127           |            |
| HD 8556   | Trilling07  | 46.6          | AB        | 2     | 0.199     | 9.28         | 0.93    | 8.96            |            |
| HD 8997   | Drake       | 23.4          | AB        |       |           |              |         | 0.09            |            |
| HD 10009  | Trilling07  | 40.4          | AB        | 2     | 0.292     | 11.79        | 0.748   | 3.82            |            |
| HD 10307  | Rodriguez15 | 12.7          | AB        | 4     | 0.631     | 8.04         | 0.434   | 7.4             | 0.43       |
| HD 10361  | Rodriguez15 | 7.8           | AB        |       |           |              |         | 86.4            |            |
| HD 10453  | Trilling07  | 39.4          | AB        | 4     | 2.5       | 98.62        | 0.919   | 78.3            |            |
| HD 10476  | Rodriguez15 | 7.5           | AB        |       |           |              |         | 0.692           |            |
| HD 11171  | Rodriguez15 | 23.2          | AB        |       |           |              |         | 4263            |            |
| HD 11636  | Rodriguez15 | 18            | AB        | 2     | 0.036     | 0.65         | 0.8801  | 0.558           |            |
| HD 11803  | Kennedy     | 39.9          | AB        | 2     | 0.986     | 39.33        | 0.726   |                 |            |
| HD 11944  | Trilling07  | 55.6          | AB        |       |           |              |         | 132             |            |
| HD 13161  | Rodriguez15 | 38.9          | AB        | 1     | 0.00802   | 0.31         | 0.44    | 0.243           | 0.43       |
| HD 13445  | Rodriguez15 | 10.8          | AB        | 5     | 4.393     | 47.37        | 0.49    | 18.22           | 0.3974     |
| HD 13594  | Trilling07  | 39.6          | AB        | 2     | 0.89      | 35.23        | 0.2626  | 37.4            |            |
| HD 13974  | Rodriguez15 | 10.8          | AB        | 1     | 0.0098    | 0.11         | 0.011   | 0.096           | 0.01       |
| HD 14082B | Rodriguez12 | 27.3          | AB        |       |           |              |         | 471.9           |            |
| HD 15285  | DUNES       | 17.1          | AB        | 1     | 0.559     | 9.58         | 0.237   |                 |            |
| HD 15814  | Drake       | 28.7          | AB        |       |           |              |         | 0.156           |            |
| HD 16160  | Rodriguez15 | 7.2           | Aa-Ab     | 9     | 0.171     | 1.23         | 0.67    |                 |            |
|           |             |               | AB        | 5     | 5.3       | 38.06        | 0.42    | 14.68           | 0.67       |
|           |             |               | AB-C      |       |           |              |         | 1186            |            |
| HD 16234  | Kennedy     | 34.7          | AB        | 1     | 0.077     | 2.67         | 0.017   |                 |            |
| HD 16555  | Rodriguez15 | 45.6          | Aa-Ab     | 2     | 0.079     | 3.6          | 0.065   | 1.05            | 0.16       |
| HD 16620  | Kennedy     | 21.5          | AB        | 1     | 0.1063    | 2.28         | 0.23    |                 |            |
| HD 16628  | Trilling07  | 71            | AB        |       |           |              |         | 2050            |            |
| HD 16754  | Rodriguez15 | 35.7          | AB-C      |       |           |              |         | 893             |            |

| Name     | Source      | Distance / pc | Component | Grade | VB6 $a / ''$ | VB6 $a / au$ | VB6 $e$ | Source $a / au$ | Source $e$ |
|----------|-------------|---------------|-----------|-------|--------------|--------------|---------|-----------------|------------|
|          |             |               | AB        |       |              |              |         |                 |            |
| HD 16765 | Rodriguez15 | 22.6          | AB        |       |              |              |         | 91              |            |
| HD 16920 | Trilling07  | 49.1          | AB        |       |              |              |         | 0.12            |            |
| HD 16970 | Rodriguez15 | 24.4          | AB        |       |              |              |         | 63.3            |            |
|          |             |               | AB-C      |       |              |              |         | 20454           |            |
| HD 17084 | Drake       | 41.1          | Aa-Ab     |       |              |              |         | 0.019           |            |
|          |             |               | AB        | 5     | 0.237        | 9.75         | 0.829   |                 |            |
| HD 17094 | Trilling07  | 25.8          | AB        |       |              |              |         | 2.58            |            |
| HD 17206 | Trilling07  | 14.2          | AB        |       |              |              |         | 2.8             |            |
| HD 17627 | Trilling07  | 56.8          | AB        |       |              |              |         | 303             |            |
| HD 17925 | Rodriguez15 | 10.4          | AB        |       |              |              |         | 0.07            |            |
| HD 18955 | Drake       | 51.2          | AB        | 2     | 0.00581      | 0.3          | 0.7594  | 0.242           |            |
| HD 19356 | Rodriguez12 | 27.6          | Aa1-Aa2   | 4     | 0.00215      | 0.06         | 0       | 0.07            |            |
|          |             |               | Aa-Ab     | 1     | 0.09343      | 2.58         | 0.227   | 3               |            |
| HD 19485 | Drake       | 77.1          | AB        |       |              |              |         | 0.073           |            |
| HD 19994 | Rodriguez15 | 22.6          | A-BC      | 5     | 6.77         | 152.86       | 0.26    | 223             | 0.26       |
|          |             |               | BC        | 7     | 0.064        | 1.45         |         |                 |            |
| HD 20010 | Rodriguez15 | 14.2          | AB        | 4     | 4            | 56.95        | 0.73    | 54.8            | 0.73       |
| HD 20320 | Rodriguez15 | 33.6          | AB        |       |              |              |         | 0.163           | 0.14       |
| HD 20631 | Trilling07  | 37            | AB        |       |              |              |         | 264             |            |
| HD 20807 | Rodriguez15 | 12            | AB        |       |              |              |         | 3717            |            |
| HD 21242 | Drake       | 50.5          | Aa-Ab     | 2     | 0.00175      | 0.09         | 0       | 0.082           |            |
|          |             |               | AB        | 5     | 0.648        | 32.71        | 0.77    | 9.402           |            |
| HD 22001 | Rodriguez15 | 21.7          | AB        |       |              |              |         | 1171            |            |
| HD 22403 | Drake       | 37            | AB        |       |              |              |         | 0.032           |            |
| HD 22694 | Drake       | 36.5          | AB        |       |              |              |         | 0.079           |            |
| HD 26354 | Drake       | 34.2          | AB        |       |              |              |         | 0.034           |            |
| HD 26690 | Trilling07  | 36.3          | AB        | 1     | 0.13302      | 4.83         | 0.3301  | 3.7             |            |
| HD 26965 | Rodriguez15 | 5             | AB        |       |              |              |         | 36.2            | 0.41       |
|          |             |               | AB-C      |       |              |              |         | 413             |            |
| HD 27149 | Drake       | 46.4          | AB        |       |              |              |         | 0.371           |            |
| HD 27710 | Trilling07  | 58.8          | AB        | 2     | 0.48         | 28.2         | 0.59    | 27.2            |            |
| HD 29140 | Trilling07  | 47.9          | Aa1-Aa2   | 9     | 0.001359     | 0.07         | 0       | 0.04            |            |
|          |             |               | Aa-Ab     | 2     | 0.2401       | 11.5         | 0.0715  | 3               |            |
|          |             |               | Ab1-Ab2   | 9     | 0.001967     | 0.09         | 0       |                 |            |
| HD 29875 | Rodriguez15 | 20.2          | AB        |       |              |              |         | 133.1           |            |
| HD 30957 | Drake       | 37.6          | AB        |       |              |              |         | 0.23            |            |
| HD 31738 | Drake       | 33.9          | AB        |       |              |              |         | 0.012           |            |
| HD 31925 | Trilling07  | 40.5          | AB        | 3     | 0.44         | 17.81        | 0.88    | 21.6            |            |
| HD 32092 | Kennedy     | 40.6          | AB        | 2     | 0.259        | 10.52        | 0.291   |                 |            |
| HD 32450 | Rodriguez15 | 8.6           | AB        | 3     | 1.062        | 9.11         | 0.72    | 8.64            |            |
| HD 32537 | Trilling07  | 26.3          | AB        |       |              |              |         | 2.62            |            |
| HD 33262 | Rodriguez15 | 11.6          | AB        |       |              |              |         | 3743            |            |
| HD 35850 | Rodriguez12 | 27            | AB        |       |              |              |         | 0.021           |            |
| HD 36705 | Rodriguez15 | 15.2          | AB        | 4     | 0.304        | 4.61         | 0.281   | 3.06            |            |
|          |             |               | A-CD      |       |              |              |         | 134.6           |            |
|          |             |               | CD        | 2     | 0.052        | 0.79         | 0.6     | 0.91            |            |
| HD 38393 | Rodriguez15 | 8.9           | AB        |       |              |              |         | 860             |            |
| HD 39891 | Trilling07  | 53.9          | AB        | 2     | 0.1117       | 6.02         | 0.537   | 5.61            |            |
| HD 42581 | Rodriguez15 | 5.8           | AB        |       |              |              |         | 44.9            |            |
| HD 43162 | Rodriguez15 | 16.7          | AB        |       |              |              |         | 411             |            |
|          |             |               | AC        |       |              |              |         | 2739            |            |
| HD 43834 | Rodriguez15 | 10.2          | AB        |       |              |              |         | 31.1            |            |
| HD 46273 | Trilling07  | 51.4          | AB        | 3     | 0.63         | 32.41        | 0.977   | 25.9            |            |
| HD 50241 | Rodriguez15 | 29.6          | AB        | 9     | 0.035        | 1.04         | 0.37    | 1.06            |            |
| HD 50635 | Trilling07  | 25.6          | AB        | 4     | 7.666        | 196.46       | 0       | 181             |            |
| HD 51199 | Trilling07  | 29.6          | AB        |       |              |              |         | 339             |            |
| HD 51733 | Trilling07  | 37.9          | AB        |       |              |              |         | 27              |            |
| HD 53705 | Rodriguez15 | 16.5          | AB        |       |              |              |         | 357             |            |
|          |             |               | AC        |       |              |              |         | 3134            |            |
| HD 54371 | Drake       | 25.2          | AB        |       |              |              |         | 0.197           |            |
| HD 56537 | Rodriguez15 | 30.9          | AB        |       |              |              |         | 297             |            |

| Name     | Source      | Distance / pc | Component | Grade | VB6 $a / ''$ | VB6 $a / au$ | VB6 $e$ | Source $a / au$ | Source $e$ |
|----------|-------------|---------------|-----------|-------|--------------|--------------|---------|-----------------|------------|
| HD 56986 | Rodriguez15 | 18.5          | AB        |       |              |              |         | 3.89            | 0.35       |
|          |             |               | AB-C      | 5     | 6.9753       | 129.32       | 0.11    | 129.6           |            |
| HD 58728 | Kennedy     | 32            | Aa1-Aa2   | 9     | 0.0005973    | 0.02         | 0.0012  |                 |            |
|          |             |               | Aa-Ab     | 2     | 0.07558      | 2.42         | 0.415   |                 |            |
| HD 58946 | Rodriguez15 | 18            | AB-C      |       |              |              |         | 61.3            |            |
|          |             |               | AB-D      |       |              |              |         | 13623           |            |
|          |             |               | AB        |       |              |              |         |                 |            |
| HD 60179 | Rodriguez15 | 15.6          | AB        |       |              |              |         | 0.12            | 0.5        |
|          |             |               | CD        |       |              |              |         | 0.052           |            |
|          |             |               | EF        | 7     | 0.00135      | 0.02         | 0       | 0.014           |            |
|          |             |               | AB-CD     | 3     | 6.755        | 105.35       | 0.336   | 94.9            |            |
|          |             |               | AB-EF     | 5     | 69.1         | 1077.67      | 0.3     | 994             |            |
| HD 60803 | Drake       | 41.5          | AB        |       |              |              |         | 0.206           |            |
| HD 61421 | Rodriguez15 | 3.5           | AB        | 3     | 4.3075       | 15.14        | 0.39785 | 13.5            | 0.41       |
| HD 61606 | Rodriguez15 | 14.2          | AB        |       |              |              |         | 827             |            |
| HD 61994 | Drake       | 29.1          | AB        | 9     | 0.0177       | 0.52         | 0.52    | 1.334           |            |
| HD 64096 | Rodriguez15 | 16.5          | AB        | 1     | 0.6179       | 10.2         | 0.7647  | 8.71            | 0.74       |
| HD 68146 | Rodriguez15 | 22.4          | A-BC      |       |              |              |         | 2059            |            |
|          |             |               | BC        |       |              |              |         |                 |            |
| HD 70958 | Trilling07  | 26.6          | AB        |       |              |              |         | 5.52            |            |
| HD 71071 | Drake       | 49.5          | AB        |       |              |              |         | 0.141           |            |
| HD 72462 | Trilling07  | 83.7          | AB        |       |              |              |         | 21.3            |            |
| HD 73752 | Rodriguez12 | 19.4          | AB        | 3     | 1.705        | 33.07        | 0.33    | 34              |            |
| HD 75632 | Rodriguez15 | 11.2          | AB        | 4     | 6.58         | 73.52        | 0.89    | 74.2            | 0.89       |
| HD 75732 | Rodriguez15 | 12.3          | AB        |       |              |              |         | 1055            |            |
| HD 76644 | Rodriguez15 | 14.5          | AB        |       |              |              |         | 6.16            | 0.36       |
|          |             |               | CD        |       |              |              |         | 10.16           | 0.35       |
|          |             |               | AB-CD     | 5     | 16.7         | 242.31       | 0.9     | 65.3            |            |
| HD 76943 | Rodriguez15 | 16.1          | AB        | 1     | 0.64566      | 10.38        | 0.15075 | 455             | 0.15       |
| HD 77137 | Drake       | 54.7          | AB        |       |              |              |         | 0.049           |            |
| HD 77190 | Trilling07  | 58            | AB        |       |              |              |         | 6100            |            |
| HD 78154 | Rodriguez15 | 20.4          | AB        | 4     | 5.8          | 118.2        | 0.801   | 73.2            |            |
| HD 78209 | Rodriguez15 | 28.8          | AB        |       |              |              |         | 0.069           | 0.2        |
| HD 79028 | Rodriguez15 | 19.6          | AB        | 9     | 0.0029       | 0.06         | 0.10636 | 0.135           | 0.09       |
| HD 79096 | Rodriguez15 | 20.4          | AB        | 1     | 0.117        | 2.38         | 0.417   | 2.36            | 0.4333     |
|          |             |               | AB-C      |       |              |              |         | 876             |            |
| HD 79210 | Rodriguez15 | 5.8           | AB        | 4     | 16.725       | 97.19        | 0.28    | 106.7           |            |
| HD 79969 | DUNES       | 17.3          | AB        | 1     | 0.68         | 11.74        | 0.32    |                 |            |
| HD 80081 | Rodriguez15 | 38.3          | A-BC      |       |              |              |         | 102.7           |            |
|          |             |               | BC        |       |              |              |         | 2.29            |            |
| HD 80441 | Trilling07  | 42.7          | AB        | 3     | 1.336        | 57           | 0.254   | 66.9            |            |
| HD 80671 | Trilling07  | 32.6          | AB        | 2     | 0.0888       | 2.9          | 0.455   | 3.35            |            |
| HD 81809 | Kennedy     | 30.4          | AB        | 2     | 0.428        | 13.02        | 0.27    |                 |            |
| HD 81858 | Kennedy     | 33.2          | AB        | 2     | 0.8599       | 28.52        | 0.5619  |                 |            |
| HD 81997 | Rodriguez15 | 17.3          | AB        |       |              |              |         | 4.44            | 0.33       |
|          |             |               | AB-C      |       |              |              |         | 1137            |            |
| HD 82328 | Rodriguez15 | 13.5          | AB        |       |              |              |         | 55.3            |            |
| HD 82434 | Kennedy     | 18.8          | AB        | 1     | 0.81         | 15.24        | 0.431   |                 |            |
| HD 82885 | Rodriguez15 | 11.4          | AB        | 5     | 3.84         | 43.66        | 0.88    | 43.6            | 0.88       |
| HD 83808 | Trilling07  | 40            | Aa-Ab     | 2     | 0.00446      | 0.18         | 0       | 0.19            |            |
| HD 85091 | Drake       | 44            | AB        |       |              |              |         | 0.046           |            |
| HD 86146 | Drake       | 28.8          | AB        |       |              |              |         | 0.103           |            |
| HD 88215 | Trilling07  | 27.7          | AB        |       |              |              |         | 0.2             |            |
| HD 89125 | Rodriguez15 | 22.8          | AB        |       |              |              |         | 168.6           |            |
| HD 90839 | Rodriguez15 | 12.8          | AB        |       |              |              |         | 7.62            | 0.8        |
|          |             |               | AB-C      |       |              |              |         | 1535            |            |
| HD 91816 | Drake       | 34.8          | AB        |       |              |              |         | 0.069           |            |
| HD 91889 | Trilling07  | 25.1          | AB        |       |              |              |         | 354             |            |
| HD 92139 | Kennedy     | 26.8          | AB        | 2     | 0.361        | 9.69         | 0.726   |                 |            |
| HD 95698 | Trilling07  | 56.1          | AB        |       |              |              |         | 5.31            |            |
| HD 96064 | Kennedy     | 26.3          | AB        | 2     | 0.343        | 9.01         | 0.119   |                 |            |
| HD 97101 | Rodriguez15 | 11.9          | AB        |       |              |              |         | 408             |            |

| Name      | Source      | Distance / pc | Component | Grade | VB6 $a / ''$ | VB6 $a / au$ | VB6 $e$ | Source $a / au$ | Source $e$ |
|-----------|-------------|---------------|-----------|-------|--------------|--------------|---------|-----------------|------------|
| HD 97584  | Rodriguez15 | 14.6          | AB        |       |              |              |         | 96.9            |            |
| HD 98231  | Rodriguez15 | 8.8           | AB        | 9     | 0.054        | 0.48         | 0.61    | 1.61            | 0.53       |
|           |             |               | AB-CD     | 1     | 2.536        | 22.4         | 0.398   | 19.74           | 0.41       |
|           |             |               | CD        |       |              |              |         | 0.047           |            |
| HD 98712  | Rodriguez15 | 13.2          | AB        | 5     | 5.896        | 77.61        | 0.63    | 59.5            |            |
| HD 99028  | Trilling07  | 23.7          | Aa-Ab     |       |              |              |         | 1.91            |            |
|           |             |               | AB        | 2     | 1.91         | 45.22        | 0.53    | 20              |            |
| HD 99211  | Rodriguez15 | 25.2          | AB        |       |              |              |         | 131.3           |            |
| HD 99491  | Rodriguez15 | 17.7          | AB        | 5     | 40.76        | 723.34       | 0.46    | 504             |            |
| HD 99565  | Kennedy     | 35.9          | AB        | 2     | 0.445        | 16           | 0.087   |                 |            |
| HD 100180 | Rodriguez15 | 23.3          | AB        | 5     | 16.25        | 379.05       | 0.2     | 357             |            |
| HD 100203 | Trilling07  | 28            | AB        | 2     | 0.79         | 22.11        | 0.4     | 22.3            |            |
| HD 100623 | Rodriguez15 | 9.6           | AB        |       |              |              |         | 162.5           |            |
| HD 101177 | Rodriguez15 | 23.3          | A-BC      | 5     | 10.33        | 240.18       | 0.05    | 214             |            |
|           |             |               | BC        |       |              |              |         | 0.157           | 0.4021     |
| HD 102365 | Rodriguez15 | 9.2           | AB        |       |              |              |         | 211             |            |
| HD 102647 | Rodriguez15 | 11            | AB        |       |              |              |         | 437             |            |
| HD 106112 | Trilling07  | 33.4          | AB        |       |              |              |         | 0.03            |            |
| HD 106516 | Rodriguez15 | 22.4          | AB        | 9     | 0.0044       | 0.1          | 0.046   | 1.96            | 0.046      |
| HD 107760 | Drake       | 43            | AB        |       |              |              |         | 0.061           |            |
| HD 108767 | Rodriguez15 | 26.6          | AB        |       |              |              |         | 644             |            |
| HD 110304 | Rodriguez15 | 39.9          | AB        | 2     | 0.869        | 34.68        | 0.793   | 25.1            | 0.79       |
| HD 110379 | Rodriguez15 | 11.7          | AB        | 2     | 3.639        | 42.52        | 0.8815  | 35.8            | 0.89       |
| HD 110833 | Rodriguez15 | 14.9          | AB        | 9     | 0.00719      | 0.11         | 0       | 0.789           |            |
|           |             |               | AB-C      |       |              |              |         | 24.3            |            |
| HD 112413 | Rodriguez15 | 35.2          | AB        |       |              |              |         | 683             |            |
| HD 112758 | Rodriguez15 | 20.9          | AB        |       |              |              |         | 0.432           |            |
|           |             |               | AB-C      |       |              |              |         | 16.68           |            |
| HD 113337 | Rodriguez12 | 36.9          | AB        |       |              |              |         | 4450.6          |            |
| HD 114378 | Rodriguez15 | 17.8          | AB        | 1     | 0.67144      | 11.97        | 0.5106  | 10.08           | 0.53       |
| HD 115383 | Rodriguez15 | 17.6          | AB        |       |              |              |         | 602             |            |
| HD 115404 | Rodriguez15 | 11.1          | AB        | 5     | 8.06         | 89.24        | 0.12    | 79.9            |            |
| HD 115953 | DUNES       | 10.7          | AB        | 2     | 1.5198       | 16.27        | 0.2148  |                 |            |
| HD 116442 | Rodriguez15 | 15.4          | AB        |       |              |              |         | 416             |            |
| HD 116656 | Rodriguez15 | 26.3          | AB        | 2     | 0.00983      | 0.26         | 0.5354  | 0.193           | 0.53       |
|           |             |               | CD        |       |              |              |         | 0.773           | 0.46       |
|           |             |               | EF        |       |              |              |         | 27.6            |            |
|           |             |               | AB-CD     | 9     | 0.78         | 20.52        | 0.6     | 362             |            |
|           |             |               | AB-EF     |       |              |              |         | 17768           |            |
| HD 118098 | Rodriguez15 | 22.7          | AB        |       |              |              |         | 25              |            |
| HD 118216 | Trilling07  | 45.7          | AB        | 9     | 0.00109      | 0.05         | 0       | 0.04            |            |
| HD 118261 | Kennedy     | 35.7          | AB        | 2     | 0.45         | 16.08        | 0.78    |                 |            |
| HD 118889 | Trilling07  | 60            | AB        | 1     | 0.19983      | 11.99        | 0.545   | 10.7            |            |
| HD 119124 | Trilling07  | 25.3          | AB        |       |              |              |         | 440             |            |
| HD 119756 | Rodriguez15 | 19.4          | AB        |       |              |              |         | 0.106           | 0.25       |
| HD 120036 | Rodriguez15 | 14.5          | AB        |       |              |              |         | 132             |            |
| HD 120136 | Rodriguez15 | 15.6          | AB        | 5     | 7.6          | 118.69       | 0.836   | 125.1           | 0.76       |
| HD 120476 | Rodriguez15 | 13.4          | AB        | 2     | 2.433        | 32.62        | 0.446   | 46.2            |            |
| HD 120690 | Rodriguez15 | 19.5          | AB        | 4     | 0.2827       | 5.51         | 0.3462  | 2.72            |            |
| HD 120987 | Trilling07  | 52.3          | AB        | 4     | 1.519        | 79.4         | 0.775   | 50.1            |            |
| HD 122742 | Rodriguez15 | 17            | AB        | 9     | 0.10528      | 1.79         | 0.547   | 4.75            | 0.48       |
| HD 125161 | Rodriguez15 | 29.1          | AB        |       |              |              |         | 1119            |            |
| HD 125276 | Rodriguez15 | 18            | AB        |       |              |              |         | 56              |            |
| HD 126660 | Rodriguez15 | 14.5          | AB        |       |              |              |         | 1005            |            |
| HD 127726 | Trilling07  | 73.6          | AB        | 1     | 0.2          | 14.73        | 0.16    | 14.3            |            |
| HD 127762 | Rodriguez12 | 26.6          | AB        |       |              |              |         | 1.8             |            |
| HD 128620 | DEBRIS      | 1.3           | AB        | 2     | 17.66        | 22.16        | 0.524   |                 |            |
| HD 128642 | Rodriguez15 | 19.9          | AB        | 9     | 0.01307      | 0.26         | 0.1478  | 0.627           |            |
| HD 129798 | Trilling07  | 40.7          | AB        |       |              |              |         | 153             |            |
| HD 130841 | Rodriguez15 | 23.2          | Aa-Ab     |       |              |              |         | 0.25            | 0.41       |
|           |             |               | BC        |       |              |              |         | 6.26            | 0.36       |
|           |             |               | A-BC      |       |              |              |         | 5362            |            |

| Name      | Source      | Distance / pc | Component | Grade | VB6 $a / ''$ | VB6 $a / au$ | VB6 $e$ | Source $a / au$ | Source $e$ |
|-----------|-------------|---------------|-----------|-------|--------------|--------------|---------|-----------------|------------|
| HD 130948 | Rodriguez15 | 18.2          | A-BC      | 5     | 52.7         | 957.66       | 0.61    | 48              |            |
|           |             |               | BC        | 3     | 0.1245       | 2.26         | 0.176   | 2.19            | 0.16       |
| HD 131156 | Rodriguez15 | 6.7           | AB        | 2     | 4.94         | 33.16        | 0.51    | 36.2            | 0.51       |
| HD 131511 | Rodriguez15 | 11.5          | AB        | 9     | 0.01652      | 0.19         | 0.51    | 0.487           | 0.51       |
| HD 131977 | Rodriguez15 | 5.8           | BC        | 3     | 0.1507       | 0.88         | 0.7559  | 0.877           | 0.76       |
|           |             |               | A-BC      | 5     | 32.34        | 188.88       | 0.2     | 141.8           |            |
|           |             |               | AD        |       |              |              |         | 1512            |            |
| HD 133640 | Rodriguez15 | 12.5          | A-BC      | 2     | 3.666        | 45.85        | 0.5111  | 36.6            | 0.55       |
|           |             |               | BC        |       |              |              |         | 0.009           |            |
| HD 133822 | Drake       | 41.9          | AB        |       |              |              |         | 0.137           |            |
| HD 135204 | Rodriguez15 | 17.7          | AB        |       |              |              |         | 1.77            |            |
| HD 136176 | Kennedy     | 36            | AB        | 2     | 1.21         | 43.54        | 0.6527  |                 |            |
|           |             |               | Ba-Bb     | 9     | 0.055        | 1.98         | 0.7     |                 |            |
| HD 137107 | Rodriguez15 | 17.9          | AB        | 1     | 0.86226      | 15.4         | 0.27907 | 13.21           | 0.28       |
| HD 137392 | Kennedy     | 36.1          | Ba-Bb     | 2     | 1.46         | 52.65        | 0.585   |                 |            |
| HD 137763 | Rodriguez15 | 20.6          | AB        | 2     | 0.1074       | 2.21         | 0.976   | 1.82            | 0.9752     |
|           |             |               | AB-C      |       |              |              |         | 1042            |            |
| HD 137909 | Rodriguez15 | 34.3          | AB        | 1     | 0.204008     | 6.99         | 0.53971 | 6.09            | 0.55       |
| HD 139006 | Rodriguez15 | 23            | AB        |       |              |              |         | 0.175           |            |
| HD 140436 | Rodriguez15 | 44.8          | AB        | 2     | 0.729        | 32.65        | 0.48    | 32.5            | 0.48       |
| HD 140538 | Rodriguez15 | 14.7          | AB        | 5     | 5.037        | 73.83        | 0.146   | 61.6            |            |
|           |             |               | Ba-Bb     |       |              |              |         | 3.23            |            |
| HD 141272 | Rodriguez15 | 21.3          | AB        |       |              |              |         | 379             |            |
| HD 142267 | Rodriguez15 | 17.3          | AB        |       |              |              |         | 0.565           | 0.5        |
| HD 142908 | Trilling07  | 41.6          | AB        |       |              |              |         | 3910            |            |
| HD 144579 | Rodriguez15 | 14.5          | AB        |       |              |              |         | 1020            |            |
| HD 146361 | Rodriguez15 | 21.1          | AB        | 8     | 0.001225     | 0.03         | 0       | 0.023           | 0.02       |
|           |             |               | AC        | 4     | 5.26         | 110.88       | 0.72    | 144.8           |            |
|           |             |               | AD        |       |              |              |         | 13420           |            |
| HD 147365 | Trilling07  | 26.4          | AB        |       |              |              |         | 53.6            |            |
| HD 147379 | Rodriguez15 | 10.7          | AB        |       |              |              |         | 697             |            |
| HD 147584 | Rodriguez15 | 12.1          | AB        |       |              |              |         | 0.119           | 0.06       |
| HD 148653 | DUNES       | 19.7          | AB        | 2     | 2.25         | 44.23        | 0.7584  |                 |            |
| HD 149630 | Rodriguez12 | 96.5          | AB        | 2     | 0.07621      | 7.36         | 0.5135  | 10.2            |            |
| HD 150682 | Trilling07  | 43.7          | AB        |       |              |              |         | 0.04            |            |
| HD 151613 | Trilling07  | 26.1          | AB        | 9     | 0.03926      | 1.03         | 0.72    | 1.14            |            |
| HD 153597 | Rodriguez15 | 15.3          | AB        | 9     | 0.02         | 0.31         | 0.2221  | 0.303           | 0.21       |
| HD 155876 | Rodriguez15 | 6             | AB        | 1     | 0.762        | 4.55         | 0.743   | 2.43            |            |
| HD 156164 | Rodriguez15 | 23            | AB        |       |              |              |         | 2.3             |            |
| HD 158614 | Kennedy     | 16.3          | AB        | 1     | 0.98         | 16.02        | 0.175   |                 |            |
| HD 159560 | Rodriguez15 | 30.5          | AB        |       |              |              |         | 0.267           | 0.03       |
|           |             |               | AB-C      |       |              |              |         | 1882            |            |
| HD 160269 | Rodriguez15 | 14.2          | AB        | 2     | 1.53         | 21.71        | 0.18    | 19.19           | 0.18       |
|           |             |               | AB-C      |       |              |              |         | 170.2           |            |
|           |             |               | AB-D      |       |              |              |         | 10465           |            |
| HD 160922 | Rodriguez15 | 23.2          | AB        | 8     | 0.003469     | 0.08         | 0.0022  | 0.068           | 0.04       |
| HD 162003 | Rodriguez15 | 22.8          | AB        | 5     | 31           | 707.92       | 0.28    | 691             |            |
| HD 163621 | Drake       | 31.1          | AB        |       |              |              |         | 0.042           |            |
| HD 163840 | Kennedy     | 28.2          | AB        | 2     | 0.08064      | 2.28         | 0.4165  |                 |            |
| HD 165189 | Rodriguez15 | 41.8          | AB        | 4     | 2.04         | 85.36        | 0.65    | 70              |            |
| HD 165341 | DUNES       | 5.1           | AB        | 1     | 4.526        | 23.01        | 0.5005  |                 |            |
| HD 165590 | Kennedy     | 39.4          | AB        | 2     | 0.253        | 9.98         | 0.956   |                 |            |
| HD 165777 | Rodriguez15 | 26.6          | AB        |       |              |              |         | 666             |            |
| HD 165908 | Rodriguez15 | 15.6          | AB        | 2     | 1.05         | 16.42        | 0.761   | 15.96           | 0.75       |
| HD 166181 | Drake       | 32.4          | Aa-Ab     |       |              |              |         | 0.029           |            |
|           |             |               | AB        | 9     | 0.0488       | 1.58         | 0.765   | 3.164           |            |
| HD 167425 | Rodriguez15 | 23            | AB        |       |              |              |         | 179.8           |            |
| HD 168151 | Rodriguez15 | 22.9          | AB        |       |              |              |         | 76.5            |            |
| HD 170153 | Rodriguez15 | 8.1           | Aa-Ab     |       |              |              |         | 47.1            | 0.41       |
|           |             |               | AB        | 1     | 0.1244       | 1            | 0.428   |                 |            |
| HD 171802 | Drake       | 38.8          | AB        |       |              |              |         | 0.031           |            |
| HD 172555 | Rodriguez15 | 28.5          | AB        |       |              |              |         | 1884            |            |

| Name      | Source      | Distance / pc | Component | Grade | VB6 $a / ''$ | VB6 $a / au$ | VB6 $e$  | Source $a / au$ | Source $e$ |
|-----------|-------------|---------------|-----------|-------|--------------|--------------|----------|-----------------|------------|
| HD 173608 | Trilling07  | 47.7          | AB        |       |              |              |          | 75.5            |            |
| HD 173739 | Rodriguez15 | 3.6           | AB        | 4     | 13.88        | 49.54        | 0.53     | 47              |            |
| HD 174429 | Rodriguez12 | 51.5          | Aa-Ab     | 4     | 2.4          | 123.58       | 0.991    | 19.9            |            |
| HD 176051 | Rodriguez15 | 14.9          | AB        | 2     | 1.2756       | 18.97        | 0.2667   | 16.64           | 0.25       |
| HD 176687 | Rodriguez15 | 27            | AB        | 1     | 0.489        | 13.22        | 0.211    | 13.22           | 0.211      |
| HD 177474 | Kennedy     | 17.3          | AB        | 2     | 1.896        | 32.81        | 0.32     |                 |            |
| HD 178449 | Trilling07  | 41.6          | AB        |       |              |              |          | 0.3             |            |
| HD 178450 | Drake       | 27.1          | AB        |       |              |              |          | 0.031           |            |
| HD 179094 | Drake       | 73.4          | AB        |       |              |              |          | 0.254           |            |
| HD 179930 | Rodriguez15 | 16.1          | AB        | 2     | 0.23         | 3.7          | 0.273    | 3.27            |            |
| HD 180445 | Drake       | 43.2          | Aa-Ab     |       |              |              |          | 0.035           |            |
|           |             |               | AB        |       |              |              |          | 337.842         |            |
| HD 181296 | Rodriguez12 | 48.2          | AB        |       |              |              |          | 198.9           |            |
|           |             |               | AB-C      |       |              |              |          | 20072.32401     |            |
| HD 183957 | Drake       | 12.9          | AB        |       |              |              |          | 0.078           |            |
| HD 184467 | DUNES       | 18.2          | AB        | 1     | 0.08103      | 1.48         | 0.38933  |                 |            |
| HD 185395 | Rodriguez15 | 18.3          | AB        |       |              |              |          | 77              |            |
| HD 186408 | Rodriguez15 | 21.1          | AB        | 4     | 35.242       | 742.88       | 0.863    | 835             |            |
|           |             |               | Aa-Ab     |       |              |              |          | 71.9            |            |
| HD 189340 | Kennedy     | 22.2          | AB        | 1     | 0.1514       | 3.36         | 0.605    |                 |            |
| HD 191104 | Trilling07  | 39.4          | AB        |       |              |              |          | 165             |            |
| HD 191408 | Rodriguez15 | 6             | AB        |       |              |              |          | 42.7            |            |
| HD 191692 | Rodriguez12 | 87.8          | Aa-Ab     | 1     | 0.0032       | 0.28         | 0.6      | 0.28            |            |
| HD 194943 | Trilling07  | 30.3          | AB        | 5     | 1.877        | 56.81        | 0.91     | 75.8            |            |
| HD 195434 | Drake       | 48.5          | AB        |       |              |              |          | 0.012           |            |
| HD 195725 | Trilling07  | 41.8          | AB        | 9     | 0.01979      | 0.83         | 0.03     | 4.16            |            |
| HD 196544 | Rodriguez12 | 57.9          | AB        |       |              |              |          | 0.15            |            |
| HD 196795 | DUNES       | 16.7          | Aa-Ab     | 2     | 0.1242       | 2.08         | 0.617    |                 |            |
|           |             |               | AB        | 2     | 0.855        | 14.3         | 0.118    |                 |            |
| HD 196885 | Trilling07  | 33.5          | Aa-Ab     | 5     | 0.636        | 21.32        | 0.42     |                 |            |
|           |             |               | AB        |       |              |              |          | 6330            |            |
| HD 197076 | Rodriguez15 | 20.9          | AB        |       |              |              |          | 2615            |            |
| HD 198084 | Kennedy     | 27.3          | Aa-Ab     | 2     | 0.065        | 1.77         | 0.551    |                 |            |
| HD 199532 | Trilling07  | 43.5          | AB        |       |              |              |          | 0.05            |            |
| HD 200391 | Drake       | 50.8          | AB        |       |              |              |          | 0.017           |            |
| HD 200499 | Trilling07  | 49.5          | AB        | 2     | 0.265        | 13.12        | 0.41     | 14.5            |            |
| HD 200525 | Rodriguez15 | 19.8          | AB        | 9     | 0.068        | 1.34         | 0.7      | 3.96            |            |
|           |             |               | AB-C      |       |              |              |          | 142.6           |            |
| HD 200968 | Rodriguez15 | 17.6          | AB        | 5     | 3.876        | 68.12        | 0.45     | 75.7            |            |
| HD 202275 | Rodriguez15 | 18.5          | AB        | 1     | 0.231965     | 4.29         | 0.436851 | 3.56            | 0.44       |
| HD 202444 | Kennedy     | 20.3          | AB        | 2     | 0.913        | 18.57        | 0.2392   |                 |            |
| HD 202730 | Rodriguez15 | 30.3          | AB        |       |              |              |          | 1.87            |            |
|           |             |               | AB-C      |       |              |              |          | 203             |            |
| HD 202940 | Rodriguez15 | 18            | AB        |       |              |              |          | 0.152           | 0.25       |
|           |             |               | AB-C      | 4     | 2.46         | 44.2         | 0.898    | 34.3            |            |
| HD 203454 | Drake       | 26.9          | AB        |       |              |              |          | 0.045           |            |
| HD 204188 | Trilling07  | 46.4          | AB        |       |              |              |          | 0.18            |            |
| HD 206301 | Drake       | 35.2          | AB        |       |              |              |          | 0.135           |            |
| HD 206826 | Rodriguez15 | 22.2          | AB        | 4     | 5.32         | 118.3        | 0.66     | 44.4            |            |
| HD 206860 | Rodriguez15 | 17.9          | AB        |       |              |              |          | 772             |            |
| HD 207098 | Rodriguez15 | 11.9          | AB        |       |              |              |          | 0.024           | 0.01       |
| HD 207129 | Rodriguez15 | 16            | AB        |       |              |              |          | 880             |            |
| HD 209100 | Rodriguez15 | 3.6           | A-BC      |       |              |              |          | 1456            |            |
|           |             |               | BC        |       |              |              |          | 2.65            |            |
| HD 210027 | Rodriguez15 | 11.7          | AB        | 8     | 0.010329     | 0.12         | 0.001764 | 0.104           |            |
| HD 210334 | Drake       | 42.8          | AB        |       |              |              |          | 0.037           |            |
| HD 211415 | Rodriguez15 | 13.8          | AB        |       |              |              |          | 46.9            |            |
| HD 212698 | Rodriguez15 | 20.2          | AB        |       |              |              |          | 44.5            |            |
| HD 213235 | Trilling07  | 51.9          | AB        | 2     | 0.72         | 37.34        | 0.5      | 37              |            |
| HD 213398 | Rodriguez15 | 43.8          | AB        |       |              |              |          | 1327            |            |
| HD 213845 | Rodriguez15 | 22.7          | AB        |       |              |              |          | 138.1           |            |
| HD 214850 | Kennedy     | 33.8          | AB        | 1     | 0.28798      | 9.73         | 0.73499  |                 |            |

| Name        | Source      | Distance / pc | Component | Grade | VB6 $a / ''$ | VB6 $a / \text{au}$ | VB6 $e$ | Source $a / \text{au}$ | Source $e$ |
|-------------|-------------|---------------|-----------|-------|--------------|---------------------|---------|------------------------|------------|
| HD 214953   | Rodriguez15 | 23.6          | AB        |       |              |                     |         | 177.2                  |            |
| HD 215648   | Rodriguez15 | 16.3          | AB        |       |              |                     |         | 192.3                  |            |
| HD 216956   | Rodriguez15 | 7.7           | AB        |       |              |                     |         | 57000                  |            |
|             |             |               | AC        |       |              |                     |         | 158000                 |            |
| HD 217014   | Rodriguez15 | 15.6          | AB        |       |              |                     |         | 44.8                   |            |
| HD 217166   | Kennedy     | 32.6          | AB        | 2     | 0.35         | 11.4                | 0.5     |                        |            |
| HD 217792   | Trilling07  | 29.4          | AB        | 9     | 0.00929      | 0.27                | 0.5286  | 0.7                    |            |
| HD 221503   | Rodriguez15 | 15.2          | A-BC      |       |              |                     |         | 5047                   |            |
|             |             |               | BC        |       |              |                     |         | 8.79                   |            |
| HD 222317   | Drake       | 48.1          | AB        |       |              |                     |         | 0.074                  |            |
| HD 223352   | Rodriguez15 | 42.1          | AB        |       |              |                     |         | 164.2                  |            |
|             |             |               | Ba-Bb     |       |              |                     |         | 8.42                   |            |
|             |             |               | AC        |       |              |                     |         | 3129                   |            |
| HD 224085   | Drake       | 39.4          | AB        |       |              |                     |         | 0.075                  |            |
| HD 224930   | Rodriguez15 | 12.2          | AB        | 1     | 0.83         | 10.1                | 0.38    | 3.68                   | 0.38       |
| HD 224953   | Rodriguez15 | 15.3          | AB        | 5     | 2.738        | 41.97               | 0.65    | 64.5                   |            |
| HD 237786   | Drake       | 68.3          | AB        |       |              |                     |         | 0.012                  |            |
| HIP 999     | Drake       | 44.1          | Aa-Ab     |       |              |                     |         | 0.029                  |            |
|             |             |               | AB        | 9     | 0.01839      | 0.81                | 0       | 2.597                  |            |
| HIP 1242    | Rodriguez15 | 5             | AB        | 2     | 0.3037       | 1.51                | 0.364   | 1.81                   | 0.364      |
| HIP 3121    | Drake       | 33.9          | AB        |       |              |                     |         | 0.027                  |            |
| HIP 3362    | Drake       | 21.7          | AB        |       |              |                     |         | 0.026                  |            |
| HIP 8920    | Rodriguez12 | 96.2          | AB        |       |              |                     |         | 0.047                  |            |
| HIP 11437   | Rodriguez12 | 40            | AB        |       |              |                     |         | 1015.2                 |            |
| HIP 14101   | Rodriguez15 | 9.4           | A-BC      |       |              |                     |         | 49.9                   |            |
|             |             |               | BC        |       |              |                     |         | 4.84                   |            |
| HIP 17962   | Drake       | 47.6          | AB        |       |              |                     |         | 0.012                  |            |
| HIP 31634   | Rodriguez15 | 15.4          | AB        |       |              |                     |         | 33.3                   |            |
| HIP 32349   | Calibration | 2.6           | AB        | 2     | 7.4957       | 19.77               | 0.59142 |                        |            |
| HIP 33499   | Rodriguez15 | 8             | AB        | 5     | 4.396        | 35.21               | 0.32    | 10.2                   |            |
| HIP 34603   | Rodriguez15 | 6.3           | AB        | 8     | 0.0111       | 0.07                | 0.3203  | 0.053                  | 0.34       |
| HIP 40167   | Kennedy     | 25.1          | AB        | 1     | 0.85921      | 21.55               | 0.3186  |                        |            |
|             |             |               | AB-C      | 4     | 7.7          | 193.13              | 0.24    |                        |            |
|             |             |               | Ca-Cb     | 4     | 0.3728       | 9.35                | 0.088   |                        |            |
| HIP 42220   | Rodriguez15 | 13.8          | AB        | 4     | 0.484        | 6.67                | 0.704   | 5.69                   |            |
| HIP 42748   | Rodriguez15 | 15.4          | AB        |       |              |                     |         | 1758                   |            |
| HIP 44349   | Drake       | 70.8          | AB        |       |              |                     |         | 0.017                  |            |
| HIP 52600   | Rodriguez15 | 13.9          | AB        | 4     | 1.791        | 24.92               | 0.86    | 9.33                   |            |
| HIP 54211   | Rodriguez15 | 4.8           | AB        |       |              |                     |         | 152.6                  |            |
| HIP 73470   | Rodriguez15 | 11.8          | AB        |       |              |                     |         | 4.99                   |            |
| HIP 80346   | Rodriguez15 | 8.1           | AB        | 3     | 0.2397       | 1.93                | 0.629   | 1.71                   | 0.67       |
| HIP 83945   | Rodriguez15 | 7.4           | AB        |       |              |                     |         | 0.05                   | 0.068      |
| HIP 106106  | Rodriguez15 | 6.7           | AB        |       |              |                     |         | 0.169                  | 0.374      |
| HIP 106255  | Rodriguez15 | 8.3           | AB        | 2     | 0.1448       | 1.2                 | 0.39    | 1.1                    | 0.416      |
| HIP 106335  | Drake       | 43            | AB        |       |              |                     |         | 0.042                  |            |
| HIP 116132  | Rodriguez15 | 6.2           | AB        | 5     | 6.87         | 42.47               | 0.2     | 31.5                   |            |
| GJ 65       | Rodriguez15 | 2.7           | AB        |       |              |                     |         | 5.23                   |            |
| GJ 473      | Rodriguez15 | 4.4           | AB        |       |              |                     |         | 3.98                   | 0.3        |
| GJ 747      | Rodriguez15 | 8.3           | AB        |       |              |                     |         | 2.36                   | 0.274      |
| GJ 866      | Rodriguez15 | 3.4           | AB        |       |              |                     |         | 0.02                   | 0.439      |
|             |             |               | AB-C      |       |              |                     |         | 0.74                   | 0.347      |
| GJ 1116     | Rodriguez15 | 5.3           | AB        |       |              |                     |         | 7.27                   |            |
| GJ 1230A    | Rodriguez15 | 9.9           | AB        |       |              |                     |         | 0.045                  | 0.009      |
|             |             |               | AB-C      |       |              |                     |         | 41.4                   |            |
| GJ 2005     | Rodriguez15 | 7.6           | A-BC      |       |              |                     |         | 8.58                   | 0.52       |
|             |             |               | BC        |       |              |                     |         | 3.53                   | 0.0227     |
| GJ 3454     | Rodriguez15 | 8.6           | AB        |       |              |                     |         | 7.7                    |            |
| GJ 3522     | Rodriguez15 | 6.8           | AB        |       |              |                     |         | 0.047                  | 0.014      |
|             |             |               | AB-C      |       |              |                     |         | 4.2                    |            |
| V* V789 Mon | Drake       | 37            | AB        |       |              |                     |         | 0.022                  |            |
