# Supplementary material for: A statistically significant lack of debris discs in medium separation binary systems
Source: arXiv:1907.04800 ancillary file (2019-07-11)
Supplement: Supplementary file 2 [file table2.pdf]

Full version of Table 2

| Name      | MIPS 70 $\mu\text{m}$         |                                |                                |        | PACS 70 $\mu\text{m}$         |                                |                                |        | PACS 100 $\mu\text{m}$        |                                |                                |        |
|-----------|-------------------------------|--------------------------------|--------------------------------|--------|-------------------------------|--------------------------------|--------------------------------|--------|-------------------------------|--------------------------------|--------------------------------|--------|
|           | $F_{\nu,\text{obs}}$<br>/ mJy | $\sigma_{\text{obs}}$<br>/ mJy | $F_{\nu,\text{pred}}$<br>/ mJy | $\chi$ | $F_{\nu,\text{obs}}$<br>/ mJy | $\sigma_{\text{obs}}$<br>/ mJy | $F_{\nu,\text{pred}}$<br>/ mJy | $\chi$ | $F_{\nu,\text{obs}}$<br>/ mJy | $\sigma_{\text{obs}}$<br>/ mJy | $F_{\nu,\text{pred}}$<br>/ mJy | $\chi$ |
| HD 38     | 14.78                         | 6.04                           | 8.16                           | 1.1    |                               |                                | 8.61                           |        | 1.85                          | 2.17                           | 4.26                           | -1.11  |
| HD 123    |                               |                                | 14.48                          |        | 14.47                         | 1.82                           | 15.29                          | -0.45  |                               |                                | 7.52                           |        |
| HD 661    | 3.1                           | 2.98                           | 4.04                           | -0.31  |                               |                                | 4.26                           |        |                               |                                | 2.1                            |        |
| HD 1237   | 11.81                         | 2.08                           | 9.24                           | 1.23   |                               |                                | 9.76                           |        | 4.1                           | 1.54                           | 4.82                           | -0.47  |
| HD 1326   | 30.5                          | 2.64                           | 31.1                           | -0.22  |                               |                                | 32.85                          |        | 14.74                         | 2.19                           | 16.3                           | -0.71  |
| HD 1404   | 43.82                         | 6.85                           | 13.65                          | 4.41   |                               |                                | 14.4                           |        | 25.38                         | 2.08                           | 7.04                           | 8.8    |
| HD 2475   |                               |                                | 7.81                           |        | 7.93                          | 1.67                           | 8.25                           | -0.19  |                               |                                | 4.07                           |        |
| HD 3196   | 21.17                         | 6.11                           | 24                             | -0.46  |                               |                                | 25.33                          |        | 18.25                         | 1.95                           | 12.51                          | 2.93   |
| HD 3405   |                               |                                | 5.91                           |        | 7.15                          | 2.79                           | 6.24                           | 0.33   |                               |                                | 3.08                           |        |
| HD 3443   | 19.23                         | 5.12                           | 22.4                           | -0.62  |                               |                                | 23.65                          |        | 9.38                          | 1.32                           | 11.66                          | -1.72  |
| HD 3651   | 11.78                         | 4.65                           | 21.35                          | -2.06  | 22.14                         | 2.23                           | 22.53                          | -0.18  | 6.28                          | 1.35                           | 11.12                          | -3.58  |
| HD 4391   | 19.5                          | 3.59                           | 15.66                          | 1.07   |                               |                                | 16.53                          |        | 10.61                         | 1.68                           | 8.16                           | 1.46   |
| HD 4676   | 29.8                          | 6.07                           | 23.31                          | 1.07   |                               |                                | 24.6                           |        | 16.65                         | 1.7                            | 12.09                          | 2.68   |
| HD 4747   | 2.08                          | 3.41                           | 5.99                           | -1.15  |                               |                                | 6.32                           |        | 8.76                          | 1.65                           | 3.12                           | 3.42   |
| HD 4967   | 6.91                          | 4.9                            | 4.31                           | 0.53   |                               |                                | 4.55                           |        | -1.36                         | 1.74                           | 2.25                           | -2.08  |
| HD 5303   |                               |                                | 5.62                           |        | 9.39                          | 2.25                           | 5.93                           | 1.54   |                               |                                | 2.91                           |        |
| HD 6767   | 8                             | 2.03                           | 9.82                           | -0.89  |                               |                                | 10.36                          |        |                               |                                | 5.12                           |        |
| HD 7439   | 13.97                         | 7.16                           | 19.68                          | -0.8   |                               |                                | 20.78                          |        | 13.43                         | 2.08                           | 10.17                          | 1.57   |
| HD 7700   |                               |                                | 0.89                           |        | -3.29                         | 2.26                           | 0.94                           | -1.87  |                               |                                | 0.46                           |        |
| HD 7788   | 20.51                         | 4.67                           | 22.17                          | -0.35  |                               |                                | 23.4                           |        | 13.79                         | 2.13                           | 11.48                          | 1.06   |
| HD 8224   | 10.64                         | 3.25                           | 3.9                            | 2.07   |                               |                                | 4.11                           |        |                               |                                | 2.02                           |        |
| HD 8357   |                               |                                | 8.93                           |        | 10.02                         | 1.87                           | 9.43                           | 0.31   |                               |                                | 4.66                           |        |
| HD 8556   | 12                            | 3.04                           | 8.69                           | 1.09   |                               |                                | 9.17                           |        |                               |                                | 4.48                           |        |
| HD 8997   |                               |                                | 6.04                           |        | 23.47                         | 2.41                           | 6.38                           | 7.09   |                               |                                | 3.15                           |        |
| HD 10009  | 2.15                          | 3.64                           | 8.36                           | -1.71  | 7.43                          | 2.07                           | 8.83                           | -0.67  |                               |                                | 4.33                           |        |
| HD 10307  | 38.86                         | 5.82                           | 31.76                          | 1.22   |                               |                                | 33.52                          |        | 15.69                         | 1.78                           | 16.53                          | -0.47  |
| HD 10361  | 43.09                         | 3.4                            | 27.51                          | 4.56   |                               |                                | 29.05                          |        | 10.73                         | 1.86                           | 14.32                          | -1.92  |
| HD 10453  | -5.67                         | 5.22                           | 11.49                          | -3.28  |                               |                                | 12.13                          |        |                               |                                | 5.98                           |        |
| HD 10476  | 51.25                         | 7.41                           | 38.88                          | 1.67   |                               |                                | 41.04                          |        | 19.4                          | 1.9                            | 20.25                          | -0.44  |
| HD 11171  | 61.63                         | 6.95                           | 20.98                          | 5.84   | 50.57                         | 2.95                           | 22.14                          | 9.57   | 37.77                         | 2.77                           | 10.85                          | 9.71   |
| HD 11636  | 85                            | 12.47                          | 85.48                          | -0.04  |                               |                                | 90.22                          |        | 44.07                         | 2.79                           | 44.18                          | -0.04  |
| HD 11803  |                               |                                | 11.5                           |        | 10.63                         | 2.17                           | 12.14                          | -0.69  |                               |                                | 6.05                           |        |
| HD 11944  | 8.93                          | 2.66                           | 5.08                           | 1.45   |                               |                                | 5.36                           |        |                               |                                | 2.65                           |        |
| HD 13161  | 643                           | 68.02                          | 68.71                          | 8.44   | 693.4                         | 39.55                          | 72.52                          | 15.7   | 526.7                         | 30.66                          | 35.58                          | 16.02  |
| HD 13445  | 3.44                          | 5.62                           | 18.06                          | -2.6   | 14.47                         | 1.89                           | 19.07                          | -2.42  | 8.82                          | 1.14                           | 9.41                           | -0.52  |
| HD 13594  | 5                             | 1.02                           | 8                              | -2.93  |                               |                                | 8.45                           |        |                               |                                | 4.16                           |        |
| HD 13974  | 42.07                         | 5.09                           | 40.34                          | 0.34   |                               |                                | 42.58                          |        | 22.45                         | 1.98                           | 20.99                          | 0.74   |
| HD 14082B | 43                            | 1.72                           | 2.51                           | 23.54  | 51.64                         | 4.36                           | 2.65                           | 11.23  | 41.99                         | 3.39                           | 1.31                           | 11.99  |
| HD 15285  | -4.9                          | 7.01                           | 7.69                           | -1.8   | 6.36                          | 2.75                           | 8.12                           | -0.64  | 6.4                           | 1.18                           | 4.01                           | 2.03   |
| HD 15814  |                               |                                | 11.15                          |        | 13.12                         | 2.16                           | 11.77                          | 0.63   |                               |                                | 5.8                            |        |
| HD 16160  | 32.28                         | 6.49                           | 34.8                           | -0.39  |                               |                                | 36.73                          |        | 13.5                          | 1.63                           | 18.13                          | -2.82  |
| HD 16234  |                               |                                | 13.93                          |        | 16.84                         | 1.58                           | 14.7                           | 1.34   |                               |                                | 7.2                            |        |
| HD 16555  | 3.26                          | 3.99                           | 11.58                          | -2.08  |                               |                                | 12.22                          |        | 6.09                          | 1.57                           | 6                              | 0.06   |
| HD 16620  | 35.44                         | 6.23                           | 24.47                          | 1.76   | 25.91                         | 2.11                           | 25.84                          | 0.04   |                               |                                | 12.68                          |        |
| HD 16628  | 42                            | 4.96                           | 7.6                            | 6.93   |                               |                                | 8.02                           |        |                               |                                | 3.94                           |        |
| HD 16754  | 8.39                          | 5.24                           | 12.52                          | -0.79  |                               |                                | 13.22                          |        | 5.96                          | 1.79                           | 6.52                           | -0.32  |
| HD 16765  | 9.78                          | 6.67                           | 12.36                          | -0.39  |                               |                                | 13.05                          |        | 6.9                           | 2.02                           | 6.39                           | 0.25   |
| HD 16920  | 17                            | 3.23                           | 16.82                          | 0.06   |                               |                                | 17.75                          |        |                               |                                | 8.72                           |        |
| HD 16970  | 39.5                          | 5.59                           | 39.6                           | -0.02  |                               |                                | 41.8                           |        | 15.44                         | 1.62                           | 20.49                          | -3.06  |
| HD 17084  |                               |                                | 3.69                           |        | 4.56                          | 1.89                           | 3.9                            | 0.35   |                               |                                | 1.92                           |        |

| Name     | MIPS 70 $\mu\text{m}$         |                                |                                |        | PACS 70 $\mu\text{m}$         |                                |                                |        | PACS 100 $\mu\text{m}$        |                                |                                |        |
|----------|-------------------------------|--------------------------------|--------------------------------|--------|-------------------------------|--------------------------------|--------------------------------|--------|-------------------------------|--------------------------------|--------------------------------|--------|
|          | $F_{\nu,\text{obs}}$<br>/ mJy | $\sigma_{\text{obs}}$<br>/ mJy | $F_{\nu,\text{pred}}$<br>/ mJy | $\chi$ | $F_{\nu,\text{obs}}$<br>/ mJy | $\sigma_{\text{obs}}$<br>/ mJy | $F_{\nu,\text{pred}}$<br>/ mJy | $\chi$ | $F_{\nu,\text{obs}}$<br>/ mJy | $\sigma_{\text{obs}}$<br>/ mJy | $F_{\nu,\text{pred}}$<br>/ mJy | $\chi$ |
| HD 17094 | 55.17                         | 4.7                            | 31.06                          | 5.1    |                               |                                | 32.78                          |        |                               |                                | 16.08                          |        |
| HD 17206 | 43                            | 16.09                          | 37.05                          | 0.37   |                               |                                | 39.11                          |        | 20.22                         | 1.84                           | 19.23                          | 0.53   |
| HD 17627 | 3.91                          | 2.72                           | 3.05                           | 0.32   |                               |                                | 3.22                           |        |                               |                                | 1.57                           |        |
| HD 17925 | 64.7                          | 6.97                           | 19.43                          | 6.5    | 71.09                         | 3.73                           | 20.51                          | 13.55  | 56.86                         | 3.68                           | 10.12                          | 12.69  |
| HD 18955 |                               |                                | 2                              |        | 3.29                          | 2.21                           | 2.11                           | 0.53   |                               |                                | 1.04                           |        |
| HD 19356 | 214.7                         | 13.4                           | 145.11                         | 5.16   |                               |                                | 153.17                         |        |                               |                                | 75.21                          |        |
| HD 19485 |                               |                                | 1.9                            |        | 2.75                          | 2.24                           | 2                              | 0.33   |                               |                                | 0.99                           |        |
| HD 19994 | 44.7                          | 4.19                           | 26.72                          | 4.29   |                               |                                | 28.21                          |        | 43.32                         | 3.46                           | 13.9                           | 8.5    |
| HD 20010 | 100.2                         | 7.23                           | 69.61                          | 4.21   |                               |                                | 73.49                          |        | 38.26                         | 2.73                           | 36.07                          | 0.8    |
| HD 20320 | 103                           | 10.77                          | 16.26                          | 8.05   | 97.84                         | 6.99                           | 17.16                          | 11.53  | 94.88                         | 7.73                           | 8.44                           | 11.18  |
| HD 20631 | -0.45                         | 3.27                           | 7.5                            | -2.43  |                               |                                | 7.91                           |        |                               |                                | 3.76                           |        |
| HD 20807 |                               |                                | 24.47                          |        | 32.74                         | 2.13                           | 25.83                          | 3.23   | 14.89                         | 1.28                           | 12.74                          | 1.67   |
| HD 21242 |                               |                                | 22.34                          |        | 38.84                         | 2.35                           | 23.59                          | 6.37   |                               |                                | 11.62                          |        |
| HD 22001 | 28.27                         | 2.85                           | 24.99                          | 1.15   |                               |                                | 26.38                          |        | 14.26                         | 2.18                           | 12.93                          | 0.61   |
| HD 22403 |                               |                                | 5.45                           |        | 8.67                          | 2.17                           | 5.75                           | 1.34   |                               |                                | 2.84                           |        |
| HD 22694 |                               |                                | 2.84                           |        | 7.57                          | 2.18                           | 3                              | 2.09   |                               |                                | 1.47                           |        |
| HD 26354 |                               |                                | 2.92                           |        | 3.18                          | 2.17                           | 3.08                           | 0.04   |                               |                                | 1.52                           |        |
| HD 26690 | 12                            | 1.11                           | 13.87                          | -1.66  |                               |                                | 14.64                          |        |                               |                                | 7.18                           |        |
| HD 26965 | 86.58                         | 5.02                           | 86.09                          | 0.1    |                               |                                | 90.89                          |        | 42.94                         | 2.47                           | 44.87                          | -0.78  |
| HD 27149 |                               |                                | 3.3                            |        | 7.86                          | 2.23                           | 3.49                           | 1.97   |                               |                                | 1.72                           |        |
| HD 27710 | 11                            | 4.02                           | 6.56                           | 1.1    |                               |                                | 6.92                           |        |                               |                                | 3.38                           |        |
| HD 29140 | 28                            | 3.2                            | 20.84                          | 2.2    |                               |                                | 22                             |        |                               |                                | 10.78                          |        |
| HD 29875 | 39.86                         | 4.46                           | 27.7                           | 2.72   |                               |                                | 29.24                          |        | 14.71                         | 1.94                           | 14.32                          | 0.2    |
| HD 30957 |                               |                                | 2.33                           |        | 5.05                          | 2.25                           | 2.45                           | 1.15   |                               |                                | 1.21                           |        |
| HD 31738 |                               |                                | 5.93                           |        | 4.79                          | 2.21                           | 6.26                           | -0.67  |                               |                                | 3.09                           |        |
| HD 31925 | 15.77                         | 2.19                           | 12.66                          | 1.42   | 15.75                         | 1.98                           | 13.37                          | 1.2    |                               |                                | 6.54                           |        |
| HD 32092 |                               |                                | 5.09                           |        | 4.5                           | 2.14                           | 5.37                           | -0.41  |                               |                                | 2.63                           |        |
| HD 32450 | 14.06                         | 3.12                           | 15.25                          | -0.38  |                               |                                | 16.1                           |        | 9.65                          | 1.64                           | 7.95                           | 1.04   |
| HD 32537 | 10.31                         | 4.74                           | 17.8                           | -1.58  |                               |                                | 18.79                          |        |                               |                                | 9.21                           |        |
| HD 33262 | 66.32                         | 6.72                           | 33.15                          | 4.93   |                               |                                | 34.99                          |        | 33.93                         | 2.37                           | 17.16                          | 7.04   |
| HD 35850 | 46.87                         | 5.37                           | 8.35                           | 7.17   |                               |                                | 8.81                           |        | 46.13                         | 2.64                           | 4.34                           | 15.82  |
| HD 36705 | -3.14                         | 6.08                           | 10.77                          | -2.29  |                               |                                | 11.37                          |        | 5.21                          | 1.68                           | 5.58                           | -0.22  |
| HD 38393 | 87.4                          | 5.27                           | 85.84                          | 0.3    |                               |                                | 90.61                          |        | 43.75                         | 4.48                           | 44.51                          | -0.17  |
| HD 39891 | 0.39                          | 2.78                           | 5.51                           | -1.84  |                               |                                | 5.82                           |        |                               |                                | 2.84                           |        |
| HD 42581 | 17.69                         | 2.9                            | 24.12                          | -2.22  |                               |                                | 25.49                          |        | 12.32                         | 1.72                           | 12.7                           | -0.22  |
| HD 43162 | 14.88                         | 2.55                           | 10.47                          | 1.73   |                               |                                | 11.06                          |        | 6.58                          | 0.86                           | 5.45                           | 1.31   |
| HD 43834 | 39.14                         | 5.75                           | 34.41                          | 0.82   |                               |                                | 36.32                          |        | 16.83                         | 1.72                           | 17.91                          | -0.63  |
| HD 46273 | 29                            | 5.13                           | 16.06                          | 2.52   | 16.33                         | 1.76                           | 16.95                          | -0.35  |                               |                                | 8.32                           |        |
| HD 50241 | 86.12                         | 7.28                           | 69.66                          | 2.26   |                               |                                | 73.54                          |        | 36.99                         | 2.36                           | 36.2                           | 0.34   |
| HD 50635 | 23                            | 4.1                            | 22.6                           | 0.1    |                               |                                | 23.85                          |        |                               |                                | 11.72                          |        |
| HD 51199 | 39                            | 5.7                            | 26.31                          | 2.23   |                               |                                | 27.77                          |        |                               |                                | 13.59                          |        |
| HD 51733 | 22.09                         | 2.41                           | 12.64                          | 3.92   |                               |                                | 13.34                          |        |                               |                                | 6.53                           |        |
| HD 53705 | 23.23                         | 2.78                           | 18.83                          | 1.58   |                               |                                | 19.87                          |        | 8.61                          | 3.42                           | 9.8                            | -0.35  |
| HD 54371 |                               |                                | 5.86                           |        | 10.84                         | 2.15                           | 6.19                           | 2.16   |                               |                                | 3.05                           |        |
| HD 56537 | 35.22                         | 6.83                           | 35.49                          | -0.04  |                               |                                | 37.46                          |        | 14.92                         | 1.8                            | 18.33                          | -1.88  |
| HD 56986 | 67                            | 10.35                          | 73.48                          | -0.62  |                               |                                | 77.57                          |        | 40.82                         | 2.46                           | 38.01                          | 1.06   |
| HD 58728 |                               |                                | 16.82                          |        | 18.81                         | 1.77                           | 17.76                          | 0.59   |                               |                                | 8.73                           |        |
| HD 58946 | 46.39                         | 6.77                           | 38.72                          | 1.13   |                               |                                | 40.87                          |        | 18.64                         | 5.02                           | 19.98                          | -0.27  |
| HD 60179 | 182.6                         | 10.18                          | 191.93                         | -0.89  |                               |                                | 202.56                         |        | 95.56                         | 4.35                           | 99.71                          | -0.89  |
| HD 60803 |                               |                                | 12.78                          |        | 15.87                         | 2.38                           | 13.49                          | 0.99   |                               |                                | 6.65                           |        |
| HD 61421 |                               |                                | 1351.53                        |        |                               |                                | 1426.66                        |        | 834                           | 39.96                          | 701.58                         | 2.92   |
| HD 61606 | -0.77                         | 5.65                           | 8.88                           | -1.71  |                               |                                | 9.37                           |        | 4.7                           | 1.81                           | 4.62                           | 0.05   |
| HD 61994 | 6.9                           | 6.91                           | 5.79                           | 0.16   | 6.28                          | 2.25                           | 6.11                           | 0.08   |                               |                                | 3.01                           |        |
| HD 64096 | 17.08                         | 5.57                           | 26.94                          | -1.77  |                               |                                | 28.44                          |        | 14.83                         | 1.57                           | 14.03                          | 0.51   |
| HD 68146 | 16.27                         | 2.24                           | 14.33                          | 0.87   |                               |                                | 15.12                          |        | 7.22                          | 3.62                           | 7.41                           | -0.05  |
| HD 70958 | 20.7                          | 3.38                           | 13.65                          | 2.08   |                               |                                | 14.4                           |        |                               |                                | 7.04                           |        |
| HD 71071 |                               |                                | 7.4                            |        | 5.97                          | 2.87                           | 7.81                           | -0.64  |                               |                                | 3.85                           |        |
| HD 72462 | 0                             | 2.69                           | 4.11                           | -1.53  |                               |                                | 4.34                           |        |                               |                                | 2.13                           |        |
| HD 73752 | 33.81                         | 5.43                           | 32.98                          | 0.15   |                               |                                | 34.81                          |        | 17.01                         | 1.87                           | 17.12                          | -0.06  |

| Name      | MIPS 70 $\mu\text{m}$         |                                |                                |        | PACS 70 $\mu\text{m}$         |                                |                                |        | PACS 100 $\mu\text{m}$        |                                |                                |        |
|-----------|-------------------------------|--------------------------------|--------------------------------|--------|-------------------------------|--------------------------------|--------------------------------|--------|-------------------------------|--------------------------------|--------------------------------|--------|
|           | $F_{\nu,\text{obs}}$<br>/ mJy | $\sigma_{\text{obs}}$<br>/ mJy | $F_{\nu,\text{pred}}$<br>/ mJy | $\chi$ | $F_{\nu,\text{obs}}$<br>/ mJy | $\sigma_{\text{obs}}$<br>/ mJy | $F_{\nu,\text{pred}}$<br>/ mJy | $\chi$ | $F_{\nu,\text{obs}}$<br>/ mJy | $\sigma_{\text{obs}}$<br>/ mJy | $F_{\nu,\text{pred}}$<br>/ mJy | $\chi$ |
| HD 75632  |                               |                                | 13.3                           |        |                               |                                | 14.04                          |        | 6.69                          | 1.75                           | 6.94                           | -0.14  |
| HD 75732  | 19.83                         | 3.34                           | 19.32                          | 0.15   |                               |                                | 20.4                           |        | 7.96                          | 1.62                           | 10.06                          | -1.29  |
| HD 76644  | 74.21                         | 5.93                           | 61.57                          | 2.09   |                               |                                | 64.99                          |        | 36.87                         | 2.88                           | 31.92                          | 1.68   |
| HD 76943  | 19.54                         | 26.07                          | 55.8                           | -1.39  |                               |                                | 58.9                           |        | 31.96                         | 2.14                           | 28.95                          | 1.4    |
| HD 77137  |                               |                                | 6.36                           |        | 4.1                           | 2.52                           | 6.72                           | -1.04  |                               |                                | 3.31                           |        |
| HD 77190  | 2.11                          | 2.1                            | 5.09                           | -1.41  |                               |                                | 5.37                           |        |                               |                                | 2.64                           |        |
| HD 78154  | 40.41                         | 5.57                           | 30.68                          | 1.75   |                               |                                | 32.39                          |        | 10.97                         | 2.55                           | 16                             | -1.97  |
| HD 78209  | 33.78                         | 4.42                           | 21.45                          | 2.79   |                               |                                | 22.64                          |        | 8.72                          | 1.63                           | 11.13                          | -1.48  |
| HD 79028  | 24.6                          | 5.1                            | 25.94                          | -0.26  |                               |                                | 27.38                          |        | 13.6                          | 1.52                           | 13.51                          | 0.06   |
| HD 79096  | 15.72                         | 11.66                          | 10.77                          | 0.42   |                               |                                | 11.37                          |        | 3.63                          | 2.14                           | 5.61                           | -0.92  |
| HD 79210  | 27.73                         | 2.78                           | 22.75                          | 1.78   |                               |                                | 24.02                          |        | 10.09                         | 2                              | 11.87                          | -0.89  |
| HD 79969  | 6.96                          | 11.15                          | 9.92                           | -0.27  | 14.66                         | 1.95                           | 10.48                          | 2.14   | 6.08                          | 1                              | 5.17                           | 0.91   |
| HD 80081  |                               |                                | 30.51                          |        |                               |                                | 32.21                          |        | 11.51                         | 1.94                           | 15.86                          | -2.23  |
| HD 80441  | 8.35                          | 3.31                           | 7.49                           | 0.26   |                               |                                | 7.91                           |        |                               |                                | 3.91                           |        |
| HD 80671  | 19.15                         | 2.52                           | 14.32                          | 1.91   | 16.95                         | 1.69                           | 15.11                          | 1.08   |                               |                                | 7.42                           |        |
| HD 81809  |                               |                                | 24.87                          |        | 32.6                          | 2.16                           | 26.25                          | 2.9    |                               |                                | 12.95                          |        |
| HD 81858  |                               |                                | 20.5                           |        | 21.59                         | 1.71                           | 21.64                          | -0.03  |                               |                                | 10.67                          |        |
| HD 81997  | 33.84                         | 3.58                           | 31.79                          | 0.57   |                               |                                | 33.56                          |        | 16.16                         | 2.65                           | 16.46                          | -0.11  |
| HD 82328  | 143.6                         | 10.21                          | 132.05                         | 1.12   |                               |                                | 139.39                         |        | 69.55                         | 4.09                           | 68.37                          | 0.29   |
| HD 82434  | 78.06                         | 5.32                           | 70.14                          | 1.43   | 79.07                         | 2.75                           | 74.06                          | 1.55   |                               |                                | 36.72                          |        |
| HD 82885  | -87.13                        | 51.73                          | 28.39                          | -2.23  |                               |                                | 29.97                          |        | 12.53                         | 1.79                           | 14.79                          | -1.26  |
| HD 83808  | 90.24                         | 5.41                           | 90.2                           | 0.01   |                               |                                | 95.22                          |        |                               |                                | 46.99                          |        |
| HD 85091  |                               |                                | 3.55                           |        | 3.82                          | 2.17                           | 3.75                           | 0.03   |                               |                                | 1.85                           |        |
| HD 86146  | 21.4                          | 4.68                           | 19.89                          | 0.32   | 20.65                         | 1.97                           | 21                             | -0.18  |                               |                                | 10.34                          |        |
| HD 88215  | 22.25                         | 3.63                           | 13.13                          | 2.5    |                               |                                | 13.86                          |        |                               |                                | 6.81                           |        |
| HD 89125  | 22.76                         | 12.71                          | 12.5                           | 0.81   |                               |                                | 13.19                          |        | 5.64                          | 2.13                           | 6.46                           | -0.38  |
| HD 90839  | 34.01                         | 4.2                            | 30.35                          | 0.87   |                               |                                | 32.04                          |        | 19.39                         | 1.93                           | 15.81                          | 1.85   |
| HD 91816  |                               |                                | 3.27                           |        | 6.72                          | 2.38                           | 3.45                           | 1.37   |                               |                                | 1.7                            |        |
| HD 91889  | 21.74                         | 3.11                           | 14.2                           | 2.42   |                               |                                | 14.99                          |        |                               |                                | 7.36                           |        |
| HD 92139  | 59                            | 18.01                          | 43.5                           | 0.86   | 51.85                         | 2.35                           | 45.91                          | 2.49   |                               |                                | 22.52                          |        |
| HD 95698  | 137                           | 14.59                          | 5.09                           | 9.04   | 154.3                         | 6.62                           | 5.37                           | 22.5   |                               |                                | 2.64                           |        |
| HD 96064  | 17.3                          | 6.43                           | 3.82                           | 2.1    | 3.13                          | 1.97                           | 4.03                           | -0.46  |                               |                                | 1.99                           |        |
| HD 97101  | 12.23                         | 4.91                           | 9.22                           | 0.61   | 7.85                          | 2.41                           | 9.73                           | -0.78  | 5.62                          | 0.91                           | 4.82                           | 0.88   |
| HD 97584  | 7.12                          | 4.43                           | 7.18                           | -0.01  |                               |                                | 7.58                           |        | 2.99                          | 1.73                           | 3.74                           | -0.43  |
| HD 98231  | 109.4                         | 9.77                           | 111.58                         | -0.22  |                               |                                | 117.82                         |        | 63.39                         | 2.65                           | 58.64                          | 1.75   |
| HD 98712  | 5.49                          | 3.28                           | 8.31                           | -0.86  |                               |                                | 8.77                           |        | 4.6                           | 2.09                           | 4.34                           | 0.13   |
| HD 99028  | 50                            | 4.47                           | 54.37                          | -0.96  |                               |                                | 57.38                          |        |                               |                                | 28.04                          |        |
| HD 99211  | 30                            | 5.27                           | 29.24                          | 0.14   |                               |                                | 30.87                          |        | 12.71                         | 2.09                           | 15.16                          | -1.17  |
| HD 99491  | 5.9                           | 7.39                           | 10.07                          | -0.56  |                               |                                | 10.63                          |        | 5.61                          | 1.8                            | 5.24                           | 0.2    |
| HD 99565  |                               |                                | 3.98                           |        | 6.6                           | 1.7                            | 4.21                           | 1.41   |                               |                                | 2.07                           |        |
| HD 100180 | 5.21                          | 6.06                           | 8.56                           | -0.55  |                               |                                | 9.03                           |        | 9.31                          | 1.68                           | 4.45                           | 2.9    |
| HD 100203 | 23                            | 2.2                            | 17.34                          | 2.56   | 18.71                         | 2.29                           | 18.3                           | 0.18   |                               |                                | 8.97                           |        |
| HD 100623 | 24.91                         | 2.71                           | 20.42                          | 1.65   |                               |                                | 21.56                          |        | 14.16                         | 1.42                           | 10.63                          | 2.48   |
| HD 101177 | 2.15                          | 5.63                           | 7.47                           | -0.95  |                               |                                | 7.89                           |        | 4.62                          | 1.6                            | 3.89                           | 0.45   |
| HD 102365 | 47.8                          | 4.75                           | 39.51                          | 1.74   |                               |                                | 41.71                          |        | 19.3                          | 2.23                           | 20.58                          | -0.57  |
| HD 102647 | 743                           | 37.44                          | 130.37                         | 16.36  | 787.1                         | 44.87                          | 137.61                         | 14.47  | 450                           | 26.41                          | 67.31                          | 14.49  |
| HD 106112 | 14                            | 4.04                           | 13.37                          | 0.16   |                               |                                | 14.11                          |        |                               |                                | 6.91                           |        |
| HD 106516 | 6.4                           | 6.19                           | 8.78                           | -0.38  |                               |                                | 9.26                           |        | 2.79                          | 1.73                           | 4.55                           | -1.02  |
| HD 107760 |                               |                                | 3.06                           |        | 6.55                          | 2.33                           | 3.23                           | 1.43   |                               |                                | 1.59                           |        |
| HD 108767 | 45.36                         | 5.36                           | 45.21                          | 0.03   |                               |                                | 47.73                          |        | 22.44                         | 2.24                           | 23.49                          | -0.47  |
| HD 110304 | 110.9                         | 7                              | 113.42                         | -0.36  |                               |                                | 119.75                         |        | 63.09                         | 3.37                           | 59.35                          | 1.1    |
| HD 110379 | 134.4                         | 12.04                          | 152.05                         | -1.46  |                               |                                | 160.56                         |        | 80.84                         | 4.25                           | 79.91                          | 0.22   |
| HD 110833 | 1.31                          | 4.66                           | 9.93                           | -1.85  | 9.73                          | 1.96                           | 10.48                          | -0.39  | 4.38                          | 0.83                           | 5.18                           | -0.96  |
| HD 112413 | 38.84                         | 4.61                           | 38.57                          | 0.06   |                               |                                | 40.73                          |        | 19.66                         | 2.1                            | 20.23                          | -0.27  |
| HD 112758 | -5.42                         | 5.18                           | 4.99                           | -2.01  |                               |                                | 5.27                           |        | -0.43                         | 1.71                           | 2.6                            | -1.77  |
| HD 113337 | 178.2                         | 18.23                          | 7.66                           | 9.35   | 180.8                         | 6                              | 8.09                           | 28.79  |                               |                                | 3.98                           |        |
| HD 114378 | 51.6                          | 5.72                           | 41.3                           | 1.8    |                               |                                | 43.6                           |        | 25.98                         | 2.38                           | 21.35                          | 1.94   |
| HD 115383 | 13.55                         | 5.11                           | 21.5                           | -1.55  |                               |                                | 22.69                          |        | 13.72                         | 1.16                           | 11.18                          | 2.18   |
| HD 115404 | 9.61                          | 5.42                           | 14.72                          | -0.94  | 15.66                         | 2.09                           | 15.53                          | 0.06   | 8.08                          | 0.88                           | 7.67                           | 0.47   |

| Name      | MIPS 70 $\mu\text{m}$         |                                |                                |        | PACS 70 $\mu\text{m}$         |                                |                                |        | PACS 100 $\mu\text{m}$        |                                |                                |        |
|-----------|-------------------------------|--------------------------------|--------------------------------|--------|-------------------------------|--------------------------------|--------------------------------|--------|-------------------------------|--------------------------------|--------------------------------|--------|
|           | $F_{\nu,\text{obs}}$<br>/ mJy | $\sigma_{\text{obs}}$<br>/ mJy | $F_{\nu,\text{pred}}$<br>/ mJy | $\chi$ | $F_{\nu,\text{obs}}$<br>/ mJy | $\sigma_{\text{obs}}$<br>/ mJy | $F_{\nu,\text{pred}}$<br>/ mJy | $\chi$ | $F_{\nu,\text{obs}}$<br>/ mJy | $\sigma_{\text{obs}}$<br>/ mJy | $F_{\nu,\text{pred}}$<br>/ mJy | $\chi$ |
| HD 115953 | 19.59                         | 4.64                           | 17.36                          | 0.48   | 16.01                         | 2.25                           | 18.33                          | -1.03  | 10                            | 1.28                           | 9.08                           | 0.72   |
| HD 116442 | 6.49                          | 5.88                           | 7.17                           | -0.12  |                               |                                | 7.57                           |        | 4.12                          | 1.79                           | 3.74                           | 0.21   |
| HD 116656 | 108.3                         | 7.15                           | 102.48                         | 0.81   |                               |                                | 108.16                         |        | 49.56                         | 2.93                           | 52.92                          | -1.13  |
| HD 118098 | 42.54                         | 6.19                           | 45.24                          | -0.44  |                               |                                | 47.75                          |        | 24.04                         | 2.04                           | 23.4                           | 0.31   |
| HD 118216 | 49.1                          | 4.99                           | 34.06                          | 3.01   | 48.93                         | 2.49                           | 35.96                          | 5.16   |                               |                                | 17.74                          |        |
| HD 118261 |                               |                                | 13.16                          |        | 7.75                          | 5.28                           | 13.89                          | -1.16  |                               |                                | 6.83                           |        |
| HD 118889 | 11.8                          | 5.21                           | 10                             | 0.35   |                               |                                | 10.56                          |        |                               |                                | 5.19                           |        |
| HD 119124 | 65.47                         | 4.13                           | 7.78                           | 13.97  |                               |                                | 8.21                           |        |                               |                                | 4.02                           |        |
| HD 119756 | 21.34                         | 7.7                            | 36.79                          | -2.01  |                               |                                | 38.83                          |        | 18.77                         | 1.92                           | 19.1                           | -0.17  |
| HD 120036 | 10.27                         | 6.13                           | 5.39                           | 0.8    |                               |                                | 5.69                           |        | 3.72                          | 1.69                           | 2.81                           | 0.54   |
| HD 120136 | 32.7                          | 5.78                           | 30.62                          | 0.36   |                               |                                | 32.31                          |        | 20.86                         | 3.45                           | 15.46                          | 1.56   |
| HD 120476 | 2.32                          | 4.74                           | 15.34                          | -2.74  | 10.02                         | 3.13                           | 16.19                          | -1.97  | 5.33                          | 1.18                           | 7.99                           | -2.24  |
| HD 120690 | 8.97                          | 2.79                           | 10.91                          | -0.69  | 8.14                          | 1.86                           | 11.51                          | -1.81  | 5.75                          | 0.9                            | 5.68                           | 0.07   |
| HD 120987 | 15.51                         | 5.87                           | 13.69                          | 0.31   |                               |                                | 14.46                          |        |                               |                                | 7.2                            |        |
| HD 122742 | 4.62                          | 5.49                           | 13.51                          | -1.62  | 15.01                         | 2.06                           | 14.27                          | 0.36   | 6.91                          | 0.83                           | 7.04                           | -0.16  |
| HD 125161 | 18.18                         | 3.64                           | 15.33                          | 0.78   |                               |                                | 16.19                          |        | 6.29                          | 1.95                           | 7.95                           | -0.85  |
| HD 125276 | 15.93                         | 6.2                            | 12.56                          | 0.54   | 14.22                         | 2.62                           | 13.26                          | 0.37   | 3.96                          | 1.3                            | 6.5                            | -1.94  |
| HD 126660 | 70.77                         | 6.26                           | 57.22                          | 2.15   |                               |                                | 60.4                           |        | 33.81                         | 2.9                            | 29.74                          | 1.39   |
| HD 127726 |                               |                                | 5.4                            |        | 5.23                          | 0.9                            | 5.7                            | -0.52  |                               |                                | 2.8                            |        |
| HD 127762 | 275.3                         | 14.43                          | 75.51                          | 13.83  |                               |                                | 79.71                          |        |                               |                                | 39.21                          |        |
| HD 128620 |                               |                                | 3127.82                        |        |                               |                                | 3302.03                        |        | 1609                          | 77.42                          | 1627.64                        | -0.23  |
| HD 128642 | 6.87                          | 4.51                           | 8.54                           | -0.37  | 9.53                          | 2.27                           | 9.01                           | 0.23   | 5.95                          | 0.9                            | 4.45                           | 1.67   |
| HD 129798 | -2.12                         | 4.73                           | 6.01                           | -1.72  |                               |                                | 6.35                           |        |                               |                                | 3.11                           |        |
| HD 130841 | 81.9                          | 4.5                            | 82.22                          | -0.07  |                               |                                | 86.79                          |        | 44.73                         | 2.71                           | 42.54                          | 0.79   |
| HD 130948 | 11.14                         | 2.99                           | 12.61                          | -0.49  |                               |                                | 13.32                          |        | 6.88                          | 0.79                           | 6.57                           | 0.39   |
| HD 131156 |                               |                                | 74.72                          |        |                               |                                | 78.88                          |        | 36.06                         | 2.8                            | 38.92                          | -1     |
| HD 131511 | 35.16                         | 5.86                           | 21.92                          | 2.26   | 30.87                         | 2.17                           | 23.14                          | 3.56   | 21.57                         | 3.93                           | 11.42                          | 2.58   |
| HD 131977 | 52.69                         | 4.13                           | 46.98                          | 1.38   |                               |                                | 49.6                           |        | 22.46                         | 1.6                            | 24.33                          | -1.15  |
| HD 133640 | 72.62                         | 6.03                           | 50.01                          | 3.74   |                               |                                | 52.81                          |        | 30.7                          | 2.15                           | 26.3                           | 2.03   |
| HD 133822 |                               |                                | 3.11                           |        | 2.34                          | 2.23                           | 3.28                           | -0.42  |                               |                                | 1.62                           |        |
| HD 135204 | 6.09                          | 5.97                           | 9.78                           | -0.62  |                               |                                | 10.33                          |        | 6.94                          | 1.7                            | 5.1                            | 1.09   |
| HD 136176 | 9.57                          | 3.21                           | 6.51                           | 0.95   | 8.3                           | 1.8                            | 6.87                           | 0.8    |                               |                                | 3.39                           |        |
| HD 137107 | 42                            | 6.15                           | 26.44                          | 2.53   |                               |                                | 27.91                          |        | 13.84                         | 2.02                           | 13.75                          | 0.04   |
| HD 137392 |                               |                                | 7.53                           |        | 4.29                          | 1.42                           | 7.95                           | -2.57  |                               |                                | 3.92                           |        |
| HD 137763 |                               |                                | 8.83                           |        |                               |                                | 9.32                           |        | 4.09                          | 2.34                           | 4.61                           | -0.22  |
| HD 137909 | 40                            | 3.4                            | 36.35                          | 1.07   |                               |                                | 38.36                          |        | 21                            | 1.92                           | 18.8                           | 1.14   |
| HD 139006 | 509.5                         | 27.31                          | 95.37                          | 15.15  | 558.3                         | 31.74                          | 100.66                         | 14.41  | 252                           | 15.3                           | 49.28                          | 13.23  |
| HD 140436 | 22.71                         | 4.18                           | 23.53                          | -0.2   |                               |                                | 24.84                          |        | 8.59                          | 1.74                           | 12.22                          | -2.08  |
| HD 140538 | 12.05                         | 5.72                           | 15.72                          | -0.64  |                               |                                | 16.6                           |        | 9.24                          | 1.36                           | 8.19                           | 0.77   |
| HD 141272 | 14                            | 0.14                           | 5.14                           | 58.07  |                               |                                | 5.42                           |        | 2.11                          | 1.62                           | 2.68                           | -0.35  |
| HD 142267 | 10.78                         | 1.81                           | 11.88                          | -0.61  |                               |                                | 12.54                          |        | 5.07                          | 1.64                           | 6.18                           | -0.68  |
| HD 142908 | 33                            | 4.62                           | 11.97                          | 4.55   |                               |                                | 12.63                          |        |                               |                                | 6.21                           |        |
| HD 144579 | 12.95                         | 2.92                           | 9.87                           | 1.05   | 9.85                          | 3.3                            | 10.42                          | -0.17  | 3.35                          | 1.12                           | 5.14                           | -1.59  |
| HD 146361 | 28.28                         | 5.41                           | 21.58                          | 1.24   |                               |                                | 22.78                          |        | 10.47                         | 2.17                           | 11.21                          | -0.34  |
| HD 147365 | 13                            | 2.07                           | 13.38                          | -0.18  |                               |                                | 14.12                          |        |                               |                                | 6.93                           |        |
| HD 147379 | 17.1                          | 5.13                           | 9.2                            | 1.54   |                               |                                | 9.71                           |        | 1.61                          | 1.93                           | 4.8                            | -1.65  |
| HD 147584 |                               |                                | 30.72                          |        |                               |                                | 32.43                          |        | 14.16                         | 1.6                            | 15.99                          | -1.14  |
| HD 148653 | 4.14                          | 4.89                           | 8.62                           | -0.92  | 10.52                         | 2.52                           | 9.1                            | 0.57   | 4.97                          | 1.09                           | 4.48                           | 0.45   |
| HD 149630 | 29.2                          | 4.7                            | 16.01                          | 2.8    |                               |                                | 16.9                           |        |                               |                                | 8.27                           |        |
| HD 150682 | 30                            | 3.66                           | 8.68                           | 5.82   |                               |                                | 9.16                           |        |                               |                                | 4.51                           |        |
| HD 151613 | 35                            | 4.69                           | 22.77                          | 2.6    |                               |                                | 24.03                          |        |                               |                                | 11.75                          |        |
| HD 153597 | 47.22                         | 5.47                           | 29.29                          | 3.28   |                               |                                | 30.92                          |        | 15.9                          | 1.13                           | 15.13                          | 0.68   |
| HD 155876 | 12.34                         | 2.98                           | 14.36                          | -0.68  |                               |                                | 15.17                          |        | 6.61                          | 0.69                           | 7.49                           | -1.27  |
| HD 156164 | 57.45                         | 5.6                            | 56.18                          | 0.23   |                               |                                | 59.3                           |        | 34.92                         | 2.25                           | 29.19                          | 2.52   |
| HD 158614 |                               |                                | 27.51                          |        | 28.2                          | 1.91                           | 29.04                          | -0.44  |                               |                                | 14.32                          |        |
| HD 159560 | 24.78                         | 3.75                           | 16.04                          | 2.33   |                               |                                | 16.93                          |        | 7.88                          | 2.86                           | 8.32                           | -0.15  |
| HD 160269 | 30.44                         | 4.86                           | 27.47                          | 0.61   |                               |                                | 29                             |        | 12.31                         | 1.34                           | 14.31                          | -1.48  |
| HD 160922 | 32.13                         | 5.46                           | 26.25                          | 1.08   |                               |                                | 27.71                          |        | 16.32                         | 1.71                           | 13.62                          | 1.58   |
| HD 162003 | 47.08                         | 5.5                            | 32.78                          | 2.6    |                               |                                | 34.6                           |        | 17.69                         | 2.68                           | 16.98                          | 0.26   |

| Name      | MIPS 70 $\mu\text{m}$         |                                |                                |        | PACS 70 $\mu\text{m}$         |                                |                                |        | PACS 100 $\mu\text{m}$        |                                |                                |        |
|-----------|-------------------------------|--------------------------------|--------------------------------|--------|-------------------------------|--------------------------------|--------------------------------|--------|-------------------------------|--------------------------------|--------------------------------|--------|
|           | $F_{\nu,\text{obs}}$<br>/ mJy | $\sigma_{\text{obs}}$<br>/ mJy | $F_{\nu,\text{pred}}$<br>/ mJy | $\chi$ | $F_{\nu,\text{obs}}$<br>/ mJy | $\sigma_{\text{obs}}$<br>/ mJy | $F_{\nu,\text{pred}}$<br>/ mJy | $\chi$ | $F_{\nu,\text{obs}}$<br>/ mJy | $\sigma_{\text{obs}}$<br>/ mJy | $F_{\nu,\text{pred}}$<br>/ mJy | $\chi$ |
| HD 163621 |                               |                                | 4.73                           |        | 7.36                          | 2.49                           | 4.99                           | 0.95   |                               |                                | 2.46                           |        |
| HD 163840 |                               |                                | 9.83                           |        | 11.7                          | 1.47                           | 10.37                          | 0.9    |                               |                                | 5.11                           |        |
| HD 165189 | 27                            | 1.08                           | 13.17                          | 12.68  |                               |                                | 13.9                           |        | 7.12                          | 2.32                           | 6.83                           | 0.13   |
| HD 165341 | 126.3                         | 8.31                           | 130.23                         | -0.44  |                               |                                | 137.48                         |        | 63.33                         | 2.44                           | 67.86                          | -1.52  |
| HD 165590 |                               |                                | 5.84                           |        | 8.3                           | 1.78                           | 6.16                           | 1.2    |                               |                                | 3.03                           |        |
| HD 165777 |                               |                                | 31.39                          |        |                               |                                | 33.13                          |        | 20.59                         | 2.15                           | 16.22                          | 2.02   |
| HD 165908 | 96.93                         | 7.09                           | 29.42                          | 9.51   | 108.2                         | 7.4                            | 31.06                          | 10.41  | 105.8                         | 7.3                            | 15.25                          | 12.41  |
| HD 166181 |                               |                                | 4.64                           |        | 9                             | 2.1                            | 4.9                            | 1.95   |                               |                                | 2.4                            |        |
| HD 167425 | 18.43                         | 5.75                           | 9.25                           | 1.6    |                               |                                | 9.76                           |        | 5                             | 1.76                           | 4.81                           | 0.1    |
| HD 168151 | 24.49                         | 3.43                           | 22.78                          | 0.5    |                               |                                | 24.05                          |        | 10.24                         | 1.59                           | 11.76                          | -0.95  |
| HD 170153 | 127.6                         | 8.13                           | 108.22                         | 2.38   |                               |                                | 114.24                         |        | 54.88                         | 3.01                           | 56.19                          | -0.43  |
| HD 171802 |                               |                                | 12.9                           |        | 12.58                         | 2.16                           | 13.62                          | -0.48  |                               |                                | 6.69                           |        |
| HD 172555 | 226.4                         | 12.79                          | 13.82                          | 16.62  | 212.8                         | 5.97                           | 14.59                          | 33.2   | 97.52                         | 5.24                           | 7.16                           | 17.24  |
| HD 173608 | 25                            | 2.66                           | 17.34                          | 2.86   | 17.6                          | 1.72                           | 18.31                          | -0.4   |                               |                                | 9.08                           |        |
| HD 173739 | 39.2                          | 4.04                           | 22.79                          | 4.05   |                               |                                | 24.08                          |        | 12.11                         | 1.16                           | 12.03                          | 0.07   |
| HD 174429 | 4.21                          | 2.79                           | 2.47                           | 0.62   | 7.08                          | 2.52                           | 2.61                           | 1.78   | 3.71                          | 2.36                           | 1.28                           | 1.02   |
| HD 176051 | 26.65                         | 5.26                           | 26.86                          | -0.04  |                               |                                | 28.36                          |        | 17.48                         | 1.87                           | 13.95                          | 1.89   |
| HD 176687 | 65.6                          | 8.02                           | 80.58                          | -1.86  |                               |                                | 85.05                          |        | 41.29                         | 2.55                           | 41.6                           | -0.12  |
| HD 177474 |                               |                                | 53.38                          |        | 63.43                         | 3.87                           | 56.35                          | 1.81   |                               |                                | 27.64                          |        |
| HD 178449 | 14                            | 1.15                           | 16.47                          | -2.12  |                               |                                | 17.38                          |        |                               |                                | 8.49                           |        |
| HD 178450 |                               |                                | 4.13                           |        | 5.11                          | 2.29                           | 4.37                           | 0.33   |                               |                                | 2.15                           |        |
| HD 179094 |                               |                                | 45.31                          |        | 52.1                          | 2.5                            | 47.84                          | 1.67   |                               |                                | 23.67                          |        |
| HD 179930 | -1.76                         | 5.01                           | 5.6                            | -1.47  |                               |                                | 5.92                           |        | 7.56                          | 1.79                           | 2.92                           | 2.59   |
| HD 180445 |                               |                                | 2.41                           |        | 7.47                          | 2.28                           | 2.55                           | 2.16   |                               |                                | 1.25                           |        |
| HD 181296 | 408.5                         | 64.79                          | 7.6                            | 6.19   |                               |                                | 8.03                           |        | 238                           | 6.83                           | 3.94                           | 34.28  |
| HD 183957 |                               |                                | 2.36                           |        | 5                             | 2.55                           | 2.49                           | 0.98   |                               |                                | 1.23                           |        |
| HD 184467 | 13.59                         | 5.25                           | 12.5                           | 0.21   | 14.91                         | 2.7                            | 13.2                           | 0.63   | 6.59                          | 0.9                            | 6.51                           | 0.08   |
| HD 185395 | 40.27                         | 3.39                           | 29.46                          | 3.14   |                               |                                | 31.09                          |        | 17.03                         | 2.13                           | 15.27                          | 0.82   |
| HD 186408 | 11                            | 6.03                           | 13.23                          | -0.37  |                               |                                | 13.97                          |        | 6.35                          | 2.31                           | 6.88                           | -0.23  |
| HD 189340 |                               |                                | 12.97                          |        | 14.51                         | 1.63                           | 13.69                          | 0.5    |                               |                                | 6.75                           |        |
| HD 191104 | 9.35                          | 3.74                           | 5.49                           | 1.03   |                               |                                | 5.8                            |        |                               |                                | 2.83                           |        |
| HD 191408 | 50.65                         | 8.89                           | 51.28                          | -0.07  |                               |                                | 54.14                          |        | 24.83                         | 1.93                           | 26.72                          | -0.97  |
| HD 191692 |                               |                                | 34.25                          |        |                               |                                | 36.15                          |        | 17.93                         | 2.98                           | 17.81                          | 0.04   |
| HD 194943 | 32                            | 5.16                           | 24.49                          | 1.45   |                               |                                | 25.85                          |        |                               |                                | 12.73                          |        |
| HD 195434 |                               |                                | 2.42                           |        | 6.74                          | 2.25                           | 2.56                           | 1.86   |                               |                                | 1.26                           |        |
| HD 195725 | 24                            | 2.22                           | 23.93                          | 0.03   |                               |                                | 25.26                          |        |                               |                                | 12.41                          |        |
| HD 196544 | 74.04                         | 10.72                          | 5.8                            | 6.37   |                               |                                | 6.12                           |        | 48.86                         | 2.24                           | 3.02                           | 20.42  |
| HD 196795 | 16.88                         | 6.08                           | 11.31                          | 0.91   | 10.73                         | 1.98                           | 11.95                          | -0.61  | 5.08                          | 1.1                            | 5.91                           | -0.75  |
| HD 196885 | 6.87                          | 3.16                           | 7.07                           | -0.06  |                               |                                | 7.46                           |        | 8.17                          | 1.17                           | 3.67                           | 3.84   |
| HD 197076 | -3.96                         | 5.2                            | 8.28                           | -2.35  |                               |                                | 8.74                           |        | 4.8                           | 2.45                           | 4.31                           | 0.2    |
| HD 198084 |                               |                                | 39.18                          |        | 44.15                         | 1.91                           | 41.36                          | 1.42   |                               |                                | 20.39                          |        |
| HD 199532 | 39.56                         | 2.82                           | 30.41                          | 3.23   |                               |                                | 32.1                           |        |                               |                                | 15.88                          |        |
| HD 200391 |                               |                                | 4.12                           |        | 4.29                          | 2.28                           | 4.35                           | -0.03  |                               |                                | 2.15                           |        |
| HD 200499 | 17                            | 3.08                           | 13.27                          | 1.21   |                               |                                | 14.01                          |        |                               |                                | 6.87                           |        |
| HD 200525 | 20.34                         | 5.2                            | 18.15                          | 0.42   |                               |                                | 19.16                          |        | 12.7                          | 1.85                           | 9.44                           | 1.76   |
| HD 200968 | -3.04                         | 5.96                           | 7.27                           | -1.73  |                               |                                | 7.67                           |        | 4.19                          | 2.35                           | 3.78                           | 0.17   |
| HD 202275 | 44.34                         | 5.14                           | 39.81                          | 0.88   |                               |                                | 42.03                          |        | 24.58                         | 2.01                           | 20.64                          | 1.96   |
| HD 202444 |                               |                                | 62.48                          |        | 81.27                         | 2.99                           | 65.95                          | 4.54   |                               |                                | 32.37                          |        |
| HD 202730 | 24.99                         | 4.76                           | 23.43                          | 0.32   |                               |                                | 24.74                          |        | 18.24                         | 2.06                           | 12.26                          | 2.88   |
| HD 202940 | 10.99                         | 6.74                           | 12.22                          | -0.18  | 11.8                          | 2.09                           | 12.9                           | -0.52  | 9.74                          | 1.04                           | 6.32                           | 3.29   |
| HD 203454 |                               |                                | 8.86                           |        | 10.99                         | 2.19                           | 9.35                           | 0.75   |                               |                                | 4.6                            |        |
| HD 204188 | 2.49                          | 2.7                            | 4.57                           | -0.77  |                               |                                | 4.83                           |        |                               |                                | 2.37                           |        |
| HD 206301 |                               |                                | 30.44                          |        | 41.68                         | 2.44                           | 32.14                          | 3.85   |                               |                                | 15.85                          |        |
| HD 206826 | 39.36                         | 5.18                           | 37.15                          | 0.42   |                               |                                | 39.22                          |        | 22.27                         | 2.12                           | 19.27                          | 1.41   |
| HD 206860 | 25.1                          | 2.85                           | 11.84                          | 4.65   |                               |                                | 12.5                           |        | 16.19                         | 1.09                           | 6.16                           | 9.19   |
| HD 207098 | 119                           | 12.91                          | 109.46                         | 0.73   |                               |                                | 115.54                         |        | 63.7                          | 3.79                           | 56.84                          | 1.77   |
| HD 207129 | 365.8                         | 19.59                          | 17.71                          | 17.77  | 316.1                         | 27.67                          | 18.7                           | 10.75  | 342.5                         | 19.87                          | 9.22                           | 16.77  |
| HD 209100 | 111.6                         | 8.24                           | 117.36                         | -0.69  |                               |                                | 123.9                          |        | 58.73                         | 2.94                           | 61.17                          | -0.82  |
| HD 210027 | 71.16                         | 6.35                           | 70.22                          | 0.15   |                               |                                | 74.11                          |        | 34.11                         | 2.25                           | 36.35                          | -0.99  |

| Name        | MIPS 70 $\mu\text{m}$         |                                |                                |        | PACS 70 $\mu\text{m}$         |                                |                                |        | PACS 100 $\mu\text{m}$        |                                |                                |        |
|-------------|-------------------------------|--------------------------------|--------------------------------|--------|-------------------------------|--------------------------------|--------------------------------|--------|-------------------------------|--------------------------------|--------------------------------|--------|
|             | $F_{\nu,\text{obs}}$<br>/ mJy | $\sigma_{\text{obs}}$<br>/ mJy | $F_{\nu,\text{pred}}$<br>/ mJy | $\chi$ | $F_{\nu,\text{obs}}$<br>/ mJy | $\sigma_{\text{obs}}$<br>/ mJy | $F_{\nu,\text{pred}}$<br>/ mJy | $\chi$ | $F_{\nu,\text{obs}}$<br>/ mJy | $\sigma_{\text{obs}}$<br>/ mJy | $F_{\nu,\text{pred}}$<br>/ mJy | $\chi$ |
| HD 210334   |                               |                                | 15.6                           |        | 21.33                         | 2.67                           | 16.47                          | 1.81   |                               |                                | 8.13                           |        |
| HD 211415   | 25.5                          | 5.73                           | 24.06                          | 0.25   |                               |                                | 25.4                           |        | 9.13                          | 1.41                           | 12.52                          | -2.39  |
| HD 212698   | 21.54                         | 5.62                           | 18.46                          | 0.55   |                               |                                | 19.49                          |        | 6.24                          | 1.77                           | 9.63                           | -1.91  |
| HD 213235   | 6.68                          | 4.79                           | 11.19                          | -0.94  |                               |                                | 11.81                          |        |                               |                                | 5.8                            |        |
| HD 213398   | 63.48                         | 4.74                           | 14.54                          | 10.31  |                               |                                | 15.35                          |        | 29.88                         | 2.44                           | 7.53                           | 9.14   |
| HD 213845   | 26.63                         | 2.96                           | 17.15                          | 3.2    |                               |                                | 18.1                           |        | 15.82                         | 1.79                           | 8.86                           | 3.88   |
| HD 214850   |                               |                                | 21.21                          |        | 21.11                         | 1.88                           | 22.39                          | -0.67  |                               |                                | 11.06                          |        |
| HD 214953   | 6.82                          | 5.25                           | 10.75                          | -0.75  |                               |                                | 11.34                          |        | 2.77                          | 2.09                           | 5.59                           | -1.34  |
| HD 215648   | 54.65                         | 4.59                           | 53.37                          | 0.28   |                               |                                | 56.34                          |        | 26.02                         | 2.12                           | 27.61                          | -0.75  |
| HD 216956   | 9057                          | 820.7                          | 305.26                         | 10.66  | 11170                         | 631.28                         | 322.19                         | 17.18  |                               |                                | 157.43                         |        |
| HD 217014   | 26.7                          | 4.63                           | 19.87                          | 1.47   |                               |                                | 20.98                          |        | 13.11                         | 3.36                           | 10.34                          | 0.82   |
| HD 217166   |                               |                                | 8.49                           |        | 7.2                           | 1.61                           | 8.96                           | -1.09  |                               |                                | 4.42                           |        |
| HD 217792   |                               |                                | 13.82                          |        | 14.51                         | 2                              | 14.59                          | -0.04  |                               |                                | 7.16                           |        |
| HD 221503   | 18.4                          | 5.73                           | 5.75                           | 2.21   |                               |                                | 6.07                           |        | 0.21                          | 1.78                           | 3                              | -1.56  |
| HD 222317   |                               |                                | 5.43                           |        | -2.88                         | 2.13                           | 5.74                           | -4.05  |                               |                                | 2.83                           |        |
| HD 223352   | 54.8                          | 7.65                           | 11.45                          | 5.67   |                               |                                | 12.08                          |        | 30.71                         | 2.75                           | 5.95                           | 9.01   |
| HD 224085   |                               |                                | 12.6                           |        | 18.79                         | 2.24                           | 13.3                           | 2.45   |                               |                                | 6.58                           |        |
| HD 224930   | 27.45                         | 5.11                           | 23.34                          | 0.8    |                               |                                | 24.64                          |        | 12.73                         | 1.13                           | 12.1                           | 0.56   |
| HD 224953   | -1.39                         | 4.93                           | 3.52                           | -1     |                               |                                | 3.72                           |        | 3.26                          | 2.25                           | 1.84                           | 0.63   |
| HD 237786   |                               |                                | 1.12                           |        | -1.16                         | 2.18                           | 1.18                           | -1.07  |                               |                                | 0.58                           |        |
| HIP 999     |                               |                                | 2.61                           |        | 4.87                          | 2.18                           | 2.75                           | 0.97   |                               |                                | 1.35                           |        |
| HIP 1242    |                               |                                | 4.63                           |        |                               |                                | 4.89                           |        | -0.39                         | 1.64                           | 2.48                           | -1.75  |
| HIP 3121    |                               |                                | 1.33                           |        | 2.81                          | 2.05                           | 1.4                            | 0.69   |                               |                                | 0.69                           |        |
| HIP 3362    |                               |                                | 3.79                           |        | 5.56                          | 1.93                           | 4                              | 0.81   |                               |                                | 1.98                           |        |
| HIP 8920    | 28.6                          | 3.1                            | 0.86                           | 8.94   | 42.54                         | 2.81                           | 0.9                            | 14.8   | 17.68                         | 0.92                           | 0.45                           | 18.69  |
| HIP 11437   | 80.77                         | 7.36                           | 1.27                           | 10.8   | 74.88                         | 4.05                           | 1.34                           | 18.15  | 64.25                         | 3.12                           | 0.66                           | 20.39  |
| HIP 14101   |                               |                                | 4.27                           |        |                               |                                | 4.51                           |        | 2.66                          | 2.91                           | 2.29                           | 0.13   |
| HIP 17962   |                               |                                | 1.09                           |        | 12.6                          | 2.26                           | 1.15                           | 5.06   |                               |                                | 0.57                           |        |
| HIP 31634   |                               |                                | 5.22                           |        |                               |                                | 5.52                           |        | 2.26                          | 1.8                            | 2.73                           | -0.26  |
| HIP 32349   | 2535                          | 102.95                         | 2705.5                         | -1.51  | 2846                          | 85.46                          | 2856.32                        | -0.1   | 1418                          | 73.22                          | 1421.77                        | -0.05  |
| HIP 33499   |                               |                                | 6.43                           |        |                               |                                | 6.79                           |        | 1.48                          | 1.67                           | 3.41                           | -1.16  |
| HIP 34603   |                               |                                | 7.43                           |        |                               |                                | 7.85                           |        | 5.02                          | 1.59                           | 3.93                           | 0.68   |
| HIP 40167   |                               |                                | 39.94                          |        | 30.28                         | 4                              | 42.17                          | -2.94  |                               |                                | 21                             |        |
| HIP 42220   |                               |                                | 6.17                           |        |                               |                                | 6.51                           |        | 4.45                          | 1.73                           | 3.22                           | 0.71   |
| HIP 42748   |                               |                                | 4.82                           |        |                               |                                | 5.09                           |        | 5.03                          | 1.79                           | 2.51                           | 1.4    |
| HIP 44349   |                               |                                | 0.81                           |        | 4.2                           | 2.29                           | 0.86                           | 1.45   |                               |                                | 0.42                           |        |
| HIP 52600   | -2.45                         | 5.85                           | 6.06                           | -1.45  |                               |                                | 6.4                            |        | 2.08                          | 1.58                           | 3.16                           | -0.68  |
| HIP 54211   | 20.27                         | 4.41                           | 14.61                          | 1.28   |                               |                                | 15.43                          |        | 6.64                          | 2.14                           | 7.62                           | -0.46  |
| HIP 73470   |                               |                                | 7.48                           |        |                               |                                | 7.89                           |        | 4.81                          | 1.59                           | 3.9                            | 0.57   |
| HIP 80346   |                               |                                | 5.98                           |        |                               |                                | 6.31                           |        | 3.27                          | 1.55                           | 3.13                           | 0.09   |
| HIP 83945   |                               |                                | 3.92                           |        |                               |                                | 4.14                           |        | -2.34                         | 1.79                           | 2.06                           | -2.47  |
| HIP 106106  |                               |                                | 9.13                           |        |                               |                                | 9.64                           |        | 4.37                          | 1.54                           | 4.78                           | -0.27  |
| HIP 106255  |                               |                                | 4.85                           |        |                               |                                | 5.13                           |        | 3.25                          | 1.6                            | 2.63                           | 0.38   |
| HIP 106335  |                               |                                | 1.31                           |        | 4.87                          | 2.37                           | 1.38                           | 1.47   |                               |                                | 0.68                           |        |
| HIP 116132  |                               |                                | 13.63                          |        |                               |                                | 14.41                          |        | 8.2                           | 1.7                            | 7.3                            | 0.52   |
| GJ 65       | 4.79                          | 2.08                           | 12.47                          | -3.69  |                               |                                | 13.19                          |        | 7.12                          | 1.63                           | 6.83                           | 0.18   |
| GJ 473      | 3.96                          | 2.71                           | 6.65                           | -0.99  |                               |                                | 7.03                           |        | 4.36                          | 1.71                           | 3.66                           | 0.41   |
| GJ 747      |                               |                                | 3.67                           |        |                               |                                | 3.87                           |        | 0.02                          | 1.45                           | 1.92                           | -1.28  |
| GJ 866      | 3.34                          | 2.52                           | 10.01                          | -2.64  |                               |                                | 10.59                          |        | 5.04                          | 1.59                           | 5.59                           | -0.35  |
| GJ 1116     |                               |                                | 3.47                           |        |                               |                                | 3.67                           |        | 3.58                          | 1.57                           | 1.91                           | 1.06   |
| GJ 1230A    |                               |                                | 3.59                           |        |                               |                                | 3.79                           |        | 2.8                           | 1.59                           | 1.96                           | 0.53   |
| GJ 2005     |                               |                                | 1.27                           |        |                               |                                | 1.34                           |        | 1.82                          | 1.73                           | 0.7                            | 0.65   |
| GJ 3454     |                               |                                | 3.14                           |        |                               |                                | 3.32                           |        | 2.49                          | 1.46                           | 1.73                           | 0.51   |
| GJ 3522     |                               |                                | 8.42                           |        |                               |                                | 8.9                            |        | 1.62                          | 1.62                           | 4.45                           | -1.75  |
| V* V789 Mon |                               |                                | 2.38                           |        | 4.27                          | 1.95                           | 2.51                           | 0.9    |                               |                                | 1.25                           |        |
